# Supplementary material for: How Technology Impacts and Compares to Humans in Socially Consequential Arenas
Source: arXiv:2211.03554 source file (2022-11-02)
Supplement: Supplementary file 1 [file appendix.tex]

\appendix
\section{Advertisements}
\label{sec:ad texts}
The full text of the 14 ad campaigns are included here for clarity:

\begin{enumerate}
    \item Get notified of COVID exposure. 
    \item Get notified of COVID exposure, without harming your privacy.
    \item Get notified of COVID exposure. App data stays on your device.
    \item Get notified of COVID exposure. You control the data you share.
    \item Get notified of COVID exposure. CovidDefense uses information about who you have been near, without harming your privacy.
    \item Get notified of COVID exposure. CovidDefense uses information about who you have been near. App data stays on your device.
    \item Get notified of COVID exposure. CovidDefense uses information about who you have been near. You control the data you share.
    \item Reduce COVID infections.
    \item Reduce COVID infections, without harming your privacy.
    \item Reduce COVID infections. App data stays on your device.
    \item Reduce COVID infections. You control the data you share.
    \item Reduce COVID infections. The app uses information about who you have been near, without harming your privacy.
    \item Reduce COVID infections. The app uses information about who you have been near. App data stays on your device.
    \item Reduce COVID infections. The app uses information about who you have been near. You control the data you share.

\end{enumerate}

\section{Datasets}

The entire dataset and model regressions can be found here: \dataset.

There are two primary datasets: one which has all 7,010,271 impressions and demographic data, and another with just the impressions that have associated geographic information. The former includes columns for Google-estimated demographics like Age and Gender, with many impressions having values of ``Unknown''. 

These two data tables for demographic and geographic impressions were represented by a row for each impression with columns for whether that impression resulted in a click; the age and gender or geography of the impression; as well as indicator variables for the presence or absence of ad information (appeals, privacy transparency -- broad privacy reassurance, non-technical control, and technical control -- and data transparency).

An associated R file is included which includes functions to reproduce each model and associated statistics.

\section{Regressions}

We report the full regression tables for all claims made in the paper. 

Table~\ref{tbl:model_all} includes overall effects for each experimental variable. These regressions are performed with all the data, just demographic data, and just geographic data. 

Table~\ref{tbl:model_all_inter} reports the interaction effect between each privacy and transparency statement with the two appeals. These regressions are performed with all the data, just demographic data, and just geographic data. 

Table~\ref{tbl:model_all_cg} reports the regression for each statement for all {\bf collective-good} ads. These regressions are performed with all the data, just demographic data, and just geographic data. 

Table~\ref{tbl:model_all_ig} reports the regression for each statement for all {\bf individual-good} ads. These regressions are performed with all the data, just demographic data, and just geographic data. 

Table~\ref{tbl:model_demo_geo} reports the regression for each experimental, demographic, and geographic variable. 

Table~\ref{tbl:model_demo_CG_Age} reports the regressions for age and gender differences for {\bf collective-good} ads.

Table~\ref{tbl:model_demo_IG_Age} reports the regressions for age and gender differences for {\bf individual-good} ads.

Table~\ref{tbl:density_inter} reports the regressions for Urban/Rural interactions with the experimental variables.

\begin{table}[!htbp] \centering 
  \caption{Modeling the five independent variables} 
  \label{tbl:model_all} 
\begin{tabular}{@{\extracolsep{5pt}}lccc} 
\\[-1.8ex]\hline 
\hline \\[-1.8ex] 
 & \multicolumn{3}{c}{\textit{Dependent variable:}} \\ 
\cline{2-4} 
\\[-1.8ex] & \multicolumn{3}{c}{Clicks} \\ 
 & All data & Just Demographic & Just Geographic \\ 
\\[-1.8ex] & (1) & (2) & (3)\\ 
\hline \\[-1.8ex] 
 Individual.Good & 0.745 & 0.730 & 0.744 \\ 
  & (0.727, 0.763) & (0.707, 0.752) & (0.726, 0.762) \\ 
  & p < 0.001$^{**}$ & p < 0.001$^{**}$ & p < 0.001$^{**}$ \\ 
  & & & \\ 
 Privacy.Broad & 1.032 & 1.031 & 1.034 \\ 
  & (0.992, 1.074) & (0.980, 1.085) & (0.993, 1.076) \\ 
  & p = 0.121 & p = 0.243 & p = 0.106 \\ 
  & & & \\ 
 NonTech.Control & 1.084 & 1.112 & 1.092 \\ 
  & (1.042, 1.128) & (1.056, 1.172) & (1.049, 1.137) \\ 
  & p = 0.0001$^{**}$ & p = 0.0001$^{**}$ & p = 0.00002$^{**}$ \\ 
  & & & \\ 
 Technical.Control & 0.920 & 0.890 & 0.924 \\ 
  & (0.883, 0.958) & (0.844, 0.938) & (0.886, 0.963) \\ 
  & p = 0.0001$^{**}$ & p = 0.00002$^{**}$ & p = 0.0002$^{**}$ \\ 
  & & & \\ 
 Data.Transparency & 0.981 & 1.028 & 0.977 \\ 
  & (0.957, 1.007) & (0.995, 1.062) & (0.953, 1.003) \\ 
  & p = 0.147 & p = 0.100 & p = 0.081 \\ 
  & & & \\ 
 Constant & 0.005 & 0.005 & 0.005 \\ 
  & (0.004, 0.005) & (0.005, 0.005) & (0.004, 0.005) \\ 
  & p < 0.001$^{**}$ & p < 0.001$^{**}$ & p < 0.001$^{**}$ \\ 
  & & & \\ 
\hline \\[-1.8ex] 
Observations & 7,010,271 & 3,920,232 & 6,858,820 \\ 
Log Likelihood & $-$182,372.500 & $-$109,490.000 & $-$178,407.300 \\ 
Akaike Inf. Crit. & 364,756.900 & 218,992.000 & 356,826.500 \\ 
\hline 
\hline \\[-1.8ex] 
\textit{Note:}  & \multicolumn{3}{r}{$^{*}$p$<$0.05; $^{**}$p$<$0.01} \\ 
\end{tabular} 
\end{table} 

\begin{table}[!htbp] \centering 
  \caption{Modeling the interaction of the appeal with the privacy and transparency statements} 
  \label{tbl:model_all_inter} 
\begin{tabular}{@{\extracolsep{5pt}}lccc} 
\\[-1.8ex]\hline 
\hline \\[-1.8ex] 
 & \multicolumn{3}{c}{\textit{Dependent variable:}} \\ 
\cline{2-4} 
\\[-1.8ex] & \multicolumn{3}{c}{Clicks} \\ 
 & All data & Just Demographic & Just Geographic \\ 
\\[-1.8ex] & (1) & (2) & (3)\\ 
\hline \\[-1.8ex] 
 Individual.Good & 0.880 & 0.763 & 0.878 \\ 
  & (0.827, 0.937) & (0.703, 0.829) & (0.824, 0.935) \\ 
  & p = 0.0001$^{**}$ & p < 0.001$^{**}$ & p = 0.0001$^{**}$ \\ 
  & & & \\ 
 Privacy.Broad & 1.106 & 1.073 & 1.110 \\ 
  & (1.048, 1.167) & (1.003, 1.147) & (1.052, 1.172) \\ 
  & p = 0.0003$^{**}$ & p = 0.041$^{*}$ & p = 0.0002$^{**}$ \\ 
  & & & \\ 
 NonTech.Control & 1.123 & 1.096 & 1.131 \\ 
  & (1.064, 1.185) & (1.026, 1.172) & (1.071, 1.195) \\ 
  & p = 0.00003$^{**}$ & p = 0.007$^{**}$ & p = 0.00001$^{**}$ \\ 
  & & & \\ 
 Technical.Control & 1.203 & 1.095 & 1.209 \\ 
  & (1.140, 1.269) & (1.025, 1.169) & (1.146, 1.277) \\ 
  & p < 0.001$^{**}$ & p = 0.008$^{**}$ & p < 0.001$^{**}$ \\ 
  & & & \\ 
 Data.Transparency & 0.911 & 0.913 & 0.904 \\ 
  & (0.881, 0.942) & (0.875, 0.952) & (0.875, 0.935) \\ 
  & p < 0.00001$^{**}$ & p = 0.00003$^{**}$ & p < 0.001$^{**}$ \\ 
  & & & \\ 
 Individual.Good:Data.Transparency & 1.185 & 1.280 & 1.194 \\ 
  & (1.126, 1.248) & (1.197, 1.369) & (1.134, 1.258) \\ 
  & p < 0.001$^{**}$ & p < 0.001$^{**}$ & p < 0.001$^{**}$ \\ 
  & & & \\ 
 Individual.Good:Privacy.Broad & 0.855 & 0.910 & 0.851 \\ 
  & (0.789, 0.927) & (0.820, 1.009) & (0.785, 0.923) \\ 
  & p = 0.0002$^{**}$ & p = 0.075 & p = 0.0002$^{**}$ \\ 
  & & & \\ 
 Individual.Good:NonTech.Control & 0.914 & 1.041 & 0.914 \\ 
  & (0.843, 0.990) & (0.934, 1.160) & (0.843, 0.991) \\ 
  & p = 0.028$^{*}$ & p = 0.469 & p = 0.030$^{*}$ \\ 
  & & & \\ 
 Individual.Good:Technical.Control & 0.515 & 0.581 & 0.514 \\ 
  & (0.473, 0.559) & (0.521, 0.648) & (0.472, 0.559) \\ 
  & p < 0.001$^{**}$ & p < 0.001$^{**}$ & p < 0.001$^{**}$ \\ 
  & & & \\ 
 Constant & 0.004 & 0.005 & 0.004 \\ 
  & (0.004, 0.004) & (0.005, 0.005) & (0.004, 0.004) \\ 
  & p < 0.001$^{**}$ & p < 0.001$^{**}$ & p < 0.001$^{**}$ \\ 
  & & & \\ 
\hline \\[-1.8ex] 
Observations & 7,010,271 & 3,920,232 & 6,858,820 \\ 
Log Likelihood & $-$182,159.100 & $-$109,357.700 & $-$178,196.900 \\ 
Akaike Inf. Crit. & 364,338.100 & 218,735.300 & 356,413.700 \\ 
\hline 
\hline \\[-1.8ex] 
\textit{Note:}  & \multicolumn{3}{r}{$^{*}$p$<$0.05; $^{**}$p$<$0.01} \\ 
\end{tabular} 
\end{table}

\begin{table}[!htbp] \centering 
  \caption{Modeling the privacy and transparency statements for Collective-Good ads} 
  \label{tbl:model_all_cg} 
\begin{tabular}{@{\extracolsep{5pt}}lccc} 
\\[-1.8ex]\hline 
\hline \\[-1.8ex] 
 & \multicolumn{3}{c}{\textit{Dependent variable:}} \\ 
\cline{2-4} 
\\[-1.8ex] & \multicolumn{3}{c}{Clicks} \\ 
 & All data & Just Demographic & Just Geographic \\ 
\\[-1.8ex] & (1) & (2) & (3)\\ 
\hline \\[-1.8ex] 
 Privacy.Broad & 1.106 & 1.073 & 1.110 \\ 
  & (1.048, 1.167) & (1.003, 1.147) & (1.052, 1.172) \\ 
  & p = 0.0003$^{**}$ & p = 0.041$^{*}$ & p = 0.0002$^{**}$ \\ 
  & & & \\ 
 NonTech.Control & 1.123 & 1.096 & 1.131 \\ 
  & (1.064, 1.185) & (1.026, 1.172) & (1.071, 1.195) \\ 
  & p = 0.00003$^{**}$ & p = 0.007$^{**}$ & p = 0.00001$^{**}$ \\ 
  & & & \\ 
 Technical.Control & 1.203 & 1.095 & 1.209 \\ 
  & (1.140, 1.269) & (1.025, 1.169) & (1.146, 1.277) \\ 
  & p < 0.001$^{**}$ & p = 0.008$^{**}$ & p < 0.001$^{**}$ \\ 
  & & & \\ 
 Data.Transparency & 0.911 & 0.913 & 0.904 \\ 
  & (0.881, 0.942) & (0.875, 0.952) & (0.875, 0.935) \\ 
  & p < 0.00001$^{**}$ & p = 0.00003$^{**}$ & p < 0.001$^{**}$ \\ 
  & & & \\ 
 Constant & 0.004 & 0.005 & 0.004 \\ 
  & (0.004, 0.004) & (0.005, 0.005) & (0.004, 0.004) \\ 
  & p < 0.001$^{**}$ & p < 0.001$^{**}$ & p < 0.001$^{**}$ \\ 
  & & & \\ 
\hline \\[-1.8ex] 
Observations & 3,523,339 & 2,027,887 & 3,446,697 \\ 
Log Likelihood & $-$102,945.400 & $-$63,818.110 & $-$100,767.200 \\ 
Akaike Inf. Crit. & 205,900.900 & 127,646.200 & 201,544.400 \\ 
\hline 
\hline \\[-1.8ex] 
\textit{Note:}  & \multicolumn{3}{r}{$^{*}$p$<$0.05; $^{**}$p$<$0.01} \\ 
\end{tabular} 
\end{table}

\begin{table}[!htbp] \centering 
  \caption{Modeling the privacy and transparency statements for Individual-Good ads} 
  \label{tbl:model_all_ig} 
\begin{tabular}{@{\extracolsep{5pt}}lccc} 
\\[-1.8ex]\hline 
\hline \\[-1.8ex] 
 & \multicolumn{3}{c}{\textit{Dependent variable:}} \\ 
\cline{2-4} 
\\[-1.8ex] & \multicolumn{3}{c}{Clicks} \\ 
 & All data & Just Demographic & Just Geographic \\ 
\\[-1.8ex] & (1) & (2) & (3)\\ 
\hline \\[-1.8ex] 
 Privacy.Broad & 0.946 & 0.976 & 0.945 \\ 
  & (0.891, 1.004) & (1.003, 1.147) & (0.890, 1.004) \\ 
  & p = 0.070 & p = 0.547 & p = 0.068 \\ 
  & & & \\ 
 NonTech.Control & 1.026 & 1.141 & 1.034 \\ 
  & (0.967, 1.089) & (1.026, 1.172) & (0.974, 1.098) \\ 
  & p = 0.396 & p = 0.003$^{**}$ & p = 0.274 \\ 
  & & & \\ 
 Technical.Control & 0.619 & 0.636 & 0.621 \\ 
  & (0.581, 0.660) & (1.025, 1.169) & (0.582, 0.663) \\ 
  & p < 0.001$^{**}$ & p < 0.001$^{**}$ & p < 0.001$^{**}$ \\ 
  & & & \\ 
 Data.Transparency & 1.080 & 1.169 & 1.080 \\ 
  & (1.038, 1.123) & (0.875, 0.952) & (1.038, 1.124) \\ 
  & p = 0.0002$^{**}$ & p < 0.001$^{**}$ & p = 0.0002$^{**}$ \\ 
  & & & \\ 
 Constant & 0.004 & 0.004 & 0.004 \\ 
  & (0.004, 0.004) & (0.005, 0.005) & (0.004, 0.004) \\ 
  & p < 0.001$^{**}$ & p < 0.001$^{**}$ & p < 0.001$^{**}$ \\ 
  & & & \\ 
\hline \\[-1.8ex] 
Observations & 3,486,932 & 1,892,345 & 3,412,123 \\ 
Log Likelihood & $-$79,213.640 & $-$45,539.550 & $-$77,429.660 \\ 
Akaike Inf. Crit. & 158,437.300 & 91,089.100 & 154,869.300 \\ 
\hline 
\hline \\[-1.8ex] 
\textit{Note:}  & \multicolumn{3}{r}{$^{*}$p$<$0.05; $^{**}$p$<$0.01} \\ 
\end{tabular} 
\end{table}

\begin{table}[!htbp] \centering 
  \caption{Modeling demographics and geographics} 
  \label{tbl:model_demo_geo}
  \resizebox*{!}{\textheight}{
\begin{tabular}{@{\extracolsep{5pt}}lcc} 
\\[-1.8ex]\hline 
\hline \\[-1.8ex] 
 & \multicolumn{2}{c}{\textit{Dependent variable:}} \\ 
\cline{2-3} 
\\[-1.8ex] & \multicolumn{2}{c}{Clicks} \\ 
 & Just Demographic & Just Geographic \\ 
\\[-1.8ex] & (1) & (2)\\ 
\hline \\[-1.8ex] 
 Age25 - 34 & 0.951 &  \\ 
  & (0.906, 0.998) &  \\ 
  & p = 0.041$^{*}$ &  \\ 
  & & \\ 
 Age35 - 44 & 0.932 &  \\ 
  & (0.886, 0.980) &  \\ 
  & p = 0.006$^{**}$ &  \\ 
  & & \\ 
 Age45 - 54 & 0.874 &  \\ 
  & (0.825, 0.925) &  \\ 
  & p = 0.00001$^{**}$ &  \\ 
  & & \\ 
 Age55 - 64 & 0.909 &  \\ 
  & (0.866, 0.954) &  \\ 
  & p = 0.0001$^{**}$ &  \\ 
  & & \\ 
 Age65+ & 1.134 &  \\ 
  & (1.077, 1.194) &  \\ 
  & p = 0.00001$^{**}$ &  \\ 
  & & \\ 
 GenderMale & 0.794 &  \\ 
  & (0.769, 0.819) &  \\ 
  & p < 0.001$^{**}$ &  \\ 
  & & \\ 
 DensityRural &  & 1.146 \\ 
  &  & (1.104, 1.189) \\ 
  &  & p < 0.001$^{**}$ \\ 
  & & \\ 
 Individual.Good & 0.747 & 0.744 \\ 
  & (0.724, 0.770) & (0.726, 0.762) \\ 
  & p < 0.001$^{**}$ & p < 0.001$^{**}$ \\ 
  & & \\ 
 Privacy.Broad & 1.014 & 1.033 \\ 
  & (0.964, 1.068) & (0.993, 1.076) \\ 
  & p = 0.584 & p = 0.110 \\ 
  & & \\ 
 NonTech.Control & 1.115 & 1.091 \\ 
  & (1.058, 1.175) & (1.048, 1.136) \\ 
  & p = 0.00005$^{**}$ & p = 0.00003$^{**}$ \\ 
  & & \\ 
 Technical.Control & 0.857 & 0.923 \\ 
  & (0.813, 0.903) & (0.886, 0.962) \\ 
  & p < 0.001$^{**}$ & p = 0.0002$^{**}$ \\ 
  & & \\ 
 Data.Transparency & 1.034 & 0.978 \\ 
  & (1.001, 1.068) & (0.953, 1.003) \\ 
  & p = 0.047$^{*}$ & p = 0.084 \\ 
  & & \\ 
 Constant & 0.006 & 0.005 \\ 
  & (0.005, 0.006) & (0.004, 0.005) \\ 
  & p < 0.001$^{**}$ & p < 0.001$^{**}$ \\ 
  & & \\ 
\hline \\[-1.8ex] 
Observations & 3,920,232 & 6,858,820 \\ 
Log Likelihood & $-$109,314.800 & $-$178,382.400 \\ 
Akaike Inf. Crit. & 218,653.500 & 356,778.700 \\ 
\hline 
\hline \\[-1.8ex] 
\textit{Note:}  & \multicolumn{2}{r}{$^{*}$p$<$0.05; $^{**}$p$<$0.01} \\ 
\end{tabular} 
}
\end{table}

\begin{table}[!htbp] \centering 
  \caption{Modeling the Age and Gender differences for Collective-Good ads} 
  \label{tbl:model_demo_CG_Age} 
\begin{tabular}{@{\extracolsep{5pt}}lccc} 
\\[-1.8ex]\hline 
\hline \\[-1.8ex] 
 & \multicolumn{3}{c}{\textit{Dependent variable:}} \\ 
\cline{2-4} 
\\[-1.8ex] & \multicolumn{3}{c}{Clicks} \\ 
 & Collective-Good & Collective-Good
Female & Collective-Good
Male \\ 
\\[-1.8ex] & (1) & (2) & (3)\\ 
\hline \\[-1.8ex] 
 Age25 - 34 & 0.902 & 0.967 & 0.849 \\ 
  & (0.849, 0.958) & (0.886, 1.055) & (0.781, 0.923) \\ 
  & p = 0.001$^{**}$ & p = 0.455 & p = 0.0002$^{**}$ \\ 
  & & & \\ 
 Age35 - 44 & 0.921 & 1.078 & 0.791 \\ 
  & (0.864, 0.981) & (0.985, 1.180) & (0.723, 0.866) \\ 
  & p = 0.012$^{*}$ & p = 0.103 & p < 0.00001$^{**}$ \\ 
  & & & \\ 
 Age45 - 54 & 0.808 & 0.952 & 0.695 \\ 
  & (0.751, 0.870) & (0.856, 1.058) & (0.627, 0.771) \\ 
  & p < 0.00001$^{**}$ & p = 0.360 & p < 0.001$^{**}$ \\ 
  & & & \\ 
 Age55 - 64 & 0.798 & 0.937 & 0.597 \\ 
  & (0.750, 0.850) & (0.865, 1.014) & (0.533, 0.669) \\ 
  & p < 0.001$^{**}$ & p = 0.106 & p < 0.001$^{**}$ \\ 
  & & & \\ 
 Age65+ & 0.969 & 1.016 & 1.021 \\ 
  & (0.906, 1.035) & (0.933, 1.105) & (0.911, 1.144) \\ 
  & p = 0.344 & p = 0.718 & p = 0.728 \\ 
  & & & \\ 
 GenderMale & 0.887 &  &  \\ 
  & (0.851, 0.924) &  &  \\ 
  & p < 0.001$^{**}$ &  &  \\ 
  & & & \\ 
 Constant & 0.006 & 0.005 & 0.006 \\ 
  & (0.006, 0.006) & (0.005, 0.006) & (0.005, 0.006) \\ 
  & p < 0.001$^{**}$ & p < 0.001$^{**}$ & p < 0.001$^{**}$ \\ 
  & & & \\ 
\hline \\[-1.8ex] 
Observations & 2,027,887 & 1,111,417 & 916,470 \\ 
Log Likelihood & $-$63,777.320 & $-$36,412.990 & $-$27,332.210 \\ 
Akaike Inf. Crit. & 127,568.600 & 72,837.980 & 54,676.420 \\ 
\hline 
\hline \\[-1.8ex] 
\textit{Note:}  & \multicolumn{3}{r}{$^{*}$p$<$0.05; $^{**}$p$<$0.01} \\ 
\end{tabular} 
\end{table} 

\begin{table}[!htbp] \centering 
  \caption{Modeling the Age and Gender differences for Individual-Good ads} 
  \label{tbl:model_demo_IG_Age} 
\begin{tabular}{@{\extracolsep{5pt}}lccc} 
\\[-1.8ex]\hline 
\hline \\[-1.8ex] 
 & \multicolumn{3}{c}{\textit{Dependent variable:}} \\ 
\cline{2-4} 
\\[-1.8ex] & \multicolumn{3}{c}{Clicks} \\ 
 & Individual-Good & Individual-Good
Female & Individual-Good
Male \\ 
\\[-1.8ex] & (1) & (2) & (3)\\ 
\hline \\[-1.8ex] 
 Age25 - 34 & 1.046 & 1.020 & 1.073 \\ 
  & (0.964, 1.134) & (0.906, 1.149) & (0.959, 1.199) \\ 
  & p = 0.280 & p = 0.740 & p = 0.218 \\ 
  & & & \\ 
 Age35 - 44 & 0.962 & 1.016 & 0.915 \\ 
  & (0.886, 1.045) & (0.903, 1.144) & (0.816, 1.027) \\ 
  & p = 0.357 & p = 0.788 & p = 0.133 \\ 
  & & & \\ 
 Age45 - 54 & 0.997 & 1.337 & 0.760 \\ 
  & (0.911, 1.091) & (1.175, 1.522) & (0.670, 0.863) \\ 
  & p = 0.947 & p = 0.00002$^{**}$ & p = 0.00003$^{**}$ \\ 
  & & & \\ 
 Age55 - 64 & 1.074 & 1.353 & 0.795 \\ 
  & (0.995, 1.160) & (1.218, 1.502) & (0.707, 0.894) \\ 
  & p = 0.068 & p < 0.00001$^{**}$ & p = 0.0002$^{**}$ \\ 
  & & & \\ 
 Age65+ & 1.331 & 1.580 & 1.065 \\ 
  & (1.227, 1.443) & (1.418, 1.760) & (0.936, 1.211) \\ 
  & p < 0.001$^{**}$ & p < 0.001$^{**}$ & p = 0.342 \\ 
  & & & \\ 
 GenderMale & 0.685 &  &  \\ 
  & (0.653, 0.719) &  &  \\ 
  & p < 0.001$^{**}$ &  &  \\ 
  & & & \\ 
 Constant & 0.004 & 0.004 & 0.003 \\ 
  & (0.004, 0.004) & (0.003, 0.004) & (0.003, 0.004) \\ 
  & p < 0.001$^{**}$ & p < 0.001$^{**}$ & p < 0.001$^{**}$ \\ 
  & & & \\ 
\hline \\[-1.8ex] 
Observations & 1,892,345 & 866,084 & 1,026,261 \\ 
Log Likelihood & $-$45,551.090 & $-$24,641.040 & $-$20,858.890 \\ 
Akaike Inf. Crit. & 91,116.180 & 49,294.090 & 41,729.780 \\ 
\hline 
\hline \\[-1.8ex] 
\textit{Note:}  & \multicolumn{3}{r}{$^{*}$p$<$0.05; $^{**}$p$<$0.01} \\ 
\end{tabular} 
\end{table}

\begin{table}[!htbp] \centering 
  \caption{Modeling the statement differences with an interaction for Density} 
  \label{tbl:density_inter} 
\resizebox{\linewidth}{!}{
\begin{tabular}{@{\extracolsep{5pt}}lccccc} 
\\[-1.8ex]\hline 
\hline \\[-1.8ex] 
 & \multicolumn{5}{c}{\textit{Dependent variable:}} \\ 
\cline{2-6} 
\\[-1.8ex] & \multicolumn{5}{c}{Clicks} \\ 
 & Appeal & Privacy: Broad & Non-Technical Control & Technical Control & Data Transparency \\ 
\\[-1.8ex] & (1) & (2) & (3) & (4) & (5)\\ 
\hline \\[-1.8ex] 
 DensityRural & 1.114 & 1.132 & 1.164 & 1.151 & 1.158 \\ 
  & (1.061, 1.170) & (1.082, 1.183) & (1.113, 1.217) & (1.103, 1.202) & (1.103, 1.216) \\ 
  & p = 0.00002$^{**}$ & p < 0.00001$^{**}$ & p < 0.0001$^{**}$ & p < 0.0001$^{**}$ & p < 0.0001$^{**}$ \\ 
  & & & & & \\ 
 Individual.Good & 0.738 &  &  &  &  \\ 
  & (0.719, 0.757) &  &  &  &  \\ 
  & p < 0.0001$^{**}$ &  &  &  &  \\ 
  & & & & & \\ 
 DensityRural:Individual.Good & 1.067 &  &  &  &  \\ 
  & (0.990, 1.150) &  &  &  &  \\ 
  & p = 0.090 &  &  &  &  \\ 
  & & & & & \\ 
 Privacy.Broad &  & 1.025 &  &  &  \\ 
  &  & (0.997, 1.054) &  &  &  \\ 
  &  & p = 0.076 &  &  &  \\ 
  & & & & & \\ 
 DensityRural:Privacy.Broad &  & 1.055 &  &  &  \\ 
  &  & (0.973, 1.143) &  &  &  \\ 
  &  & p = 0.197 &  &  &  \\ 
  & & & & & \\ 
 NonTech.Control &  &  & 1.110 &  &  \\ 
  &  &  & (1.080, 1.141) &  &  \\ 
  &  &  & p < 0.0001$^{**}$ &  &  \\ 
  & & & & & \\ 
 DensityRural:NonTech.Control &  &  & 0.959 &  &  \\ 
  &  &  & (0.884, 1.040) &  &  \\ 
  &  &  & p = 0.314 &  &  \\ 
  & & & & & \\ 
 Technical.Control &  &  &  & 0.875 &  \\ 
  &  &  &  & (0.850, 0.901) &  \\ 
  &  &  &  & p < 0.0001$^{**}$ &  \\ 
  & & & & & \\ 
 DensityRural:Technical.Control &  &  &  & 0.998 &  \\ 
  &  &  &  & (0.917, 1.086) &  \\ 
  &  &  &  & p = 0.959 &  \\ 
  & & & & & \\ 
 Data.Transparency &  &  &  &  & 0.977 \\ 
  &  &  &  &  & (0.952, 1.002) \\ 
  &  &  &  &  & p = 0.075 \\ 
  & & & & & \\ 
 DensityRural:Data.Transparency &  &  &  &  & 0.983 \\ 
  &  &  &  &  & (0.912, 1.060) \\ 
  &  &  &  &  & p = 0.656 \\ 
  & & & & & \\ 
 Constant & 0.005 & 0.004 & 0.004 & 0.004 & 0.004 \\ 
  & (0.004, 0.005) & (0.004, 0.004) & (0.004, 0.004) & (0.004, 0.004) & (0.004, 0.004) \\ 
  & p < 0.0001$^{**}$ & p < 0.0001$^{**}$ & p < 0.0001$^{**}$ & p < 0.0001$^{**}$ & p < 0.0001$^{**}$ \\ 
  & & & & & \\ 
\hline \\[-1.8ex] 
Observations & 6,858,820 & 6,858,820 & 6,858,820 & 6,858,820 & 6,858,820 \\ 
Log Likelihood & $-$178,438.100 & $-$178,732.500 & $-$178,707.500 & $-$178,688.200 & $-$178,733.900 \\ 
Akaike Inf. Crit. & 356,884.200 & 357,473.000 & 357,423.000 & 357,384.500 & 357,475.800 \\ 
\hline 
\hline \\[-1.8ex] 
\textit{Note:}  & \multicolumn{5}{r}{$^{*}$p$<$0.05; $^{**}$p$<$0.01} \\ 
\end{tabular} }
\end{table}
