# Supplementary material for: How Technology Impacts and Compares to Humans in Socially Consequential Arenas
Source: arXiv:2211.03554 source file (2022-11-02)
Supplement: Supplementary file 2 [file appendix.tex]

\section{Results Tables}\label{app:tables}

Table~\ref{tbl:human} reports the logistic regressions which depict the bias found between gender and skin type of the subject, even when controlling for respondent demographics. 

Table~\ref{tbl:machine} reports the logistic regressions which depict the bias found between gender and skin type of the subject.

The demographics of the subject in the question are represented with a q (\texttt{qgender} and \texttt{qskin\_type}). The demographics of respondent are represented with an r (\texttt{rgender} and \texttt{rskin\_type}).

\begin{table}[!htbp] \centering 
  \caption{Logistic regressions for {\bf human} performance controlling for gender and skin types (when 2 Fitzpatrick categories are used and when 3 are used)} 
  \label{tbl:human} 
\begin{tabular}{@{\extracolsep{5pt}}lcccc} 
\\[-1.8ex]\hline 
\hline \\[-1.8ex] 
 & \multicolumn{4}{c}{\textit{Dependent variable:}} \\ 
\cline{2-5} 
\\[-1.8ex] & \multicolumn{2}{c}{3 Fitz Categories} & \multicolumn{2}{c}{2 Fitz Categories} \\ 
 & Identification & Verification & Identification & Verification \\ 
\\[-1.8ex] & (1) & (2) & (3) & (4)\\ 
\hline \\[-1.8ex] 
 qgenderMale & 1.965 & 1.394 & 1.973 & 1.395 \\ 
  & t = 20.488$^{***}$ & t = 13.050$^{***}$ & t = 20.556$^{***}$ & t = 13.069$^{***}$ \\ 
  & & & & \\ 
 qskin\_type3III-IV & 0.919 & 0.931 &  &  \\ 
  & t = $-$2.065$^{**}$ & t = $-$2.273$^{**}$ &  &  \\ 
  & & & & \\ 
 qskin\_type3V-VI & 0.697 & 0.846 &  &  \\ 
  & t = $-$9.055$^{***}$ & t = $-$5.378$^{***}$ &  &  \\ 
  & & & & \\ 
 qskin\_type2dark &  &  & 0.667 & 0.779 \\ 
  &  &  & t = $-$12.341$^{***}$ & t = $-$9.846$^{***}$ \\ 
  & & & & \\ 
 rgenderMale & 0.949 & 0.895 & 0.955 & 0.896 \\ 
  & t = $-$1.591 & t = $-$4.386$^{***}$ & t = $-$1.403 & t = $-$4.325$^{***}$ \\ 
  & & & & \\ 
 rskin\_type3III-IV & 1.078 & 1.104 &  &  \\ 
  & t = 1.869$^{*}$ & t = 3.182$^{***}$ &  &  \\ 
  & & & & \\ 
 rskin\_type3V-VI & 1.215 & 1.128 &  &  \\ 
  & t = 4.944$^{***}$ & t = 3.950$^{***}$ &  &  \\ 
  & & & & \\ 
 rskin\_type2dark &  &  & 1.239 & 1.139 \\ 
  &  &  & t = 6.525$^{***}$ & t = 5.119$^{***}$ \\ 
  & & & & \\ 
 Constant & 1.734 & 3.394 & 1.789 & 3.576 \\ 
  & t = 12.960$^{***}$ & t = 36.895$^{***}$ & t = 15.985$^{***}$ & t = 44.590$^{***}$ \\ 
  & & & & \\ 
\hline \\[-1.8ex] 
Observations & 17,877 & 37,605 & 17,877 & 37,605 \\ 
Log Likelihood & $-$10,865.250 & $-$19,292.960 & $-$10,825.090 & $-$19,254.730 \\ 
Akaike Inf. Crit. & 21,744.500 & 38,599.910 & 21,660.190 & 38,519.460 \\ 
\hline 
\hline \\[-1.8ex] 
\textit{Note:}  & \multicolumn{4}{r}{$^{*}$p$<$0.1; $^{**}$p$<$0.05; $^{***}$p$<$0.01} \\ 
\end{tabular} 
\end{table}  

\begin{table}[!tbp] \centering 
  \caption{Logistic regressions for {\bf machine} performance controlling for gender and skin types (when 2 Fitzpatrick categories are used and when 3 are used)} 
  \label{tbl:machine} 
\begin{tabular}{@{\extracolsep{5pt}}lcccc} 
\\[-1.8ex]\hline 
\hline \\[-1.8ex] 
 & \multicolumn{4}{c}{\textit{Dependent variable:}} \\ 
\cline{2-5} 
\\[-1.8ex] & \multicolumn{2}{c}{3 Fitz Categories} & \multicolumn{2}{c}{2 Fitz Categories} \\ 
 & Identification & Verification & Identification & Verification \\ 
\\[-1.8ex] & (1) & (2) & (3) & (4)\\ 
\hline \\[-1.8ex] 
 qgenderMale & 1.763 & 1.279 & 1.762 & 1.282 \\ 
  & t = 5.307$^{***}$ & t = 2.116$^{**}$ & t = 5.304$^{***}$ & t = 2.141$^{**}$ \\ 
  & & & & \\ 
 qskin\_type3III-IV & 1.074 & 0.931 &  &  \\ 
  & t = 0.537 & t = $-$0.479 &  &  \\ 
  & & & & \\ 
 qskin\_type3V-VI & 0.777 & 0.673 &  &  \\ 
  & t = $-$2.038$^{**}$ & t = $-$2.825$^{***}$ &  &  \\ 
  & & & & \\ 
 qskin\_type2dark &  &  & 0.867 & 0.762 \\ 
  &  &  & t = $-$1.371 & t = $-$2.331$^{**}$ \\ 
  & & & & \\ 
 Constant & 10.313 & 16.876 & 10.361 & 16.431 \\ 
  & t = 23.163$^{***}$ & t = 23.625$^{***}$ & t = 27.235$^{***}$ & t = 27.569$^{***}$ \\ 
  & & & & \\ 
\hline \\[-1.8ex] 
Observations & 5,406 & 5,430 & 5,406 & 5,430 \\ 
Log Likelihood & $-$1,423.145 & $-$1,209.350 & $-$1,425.953 & $-$1,211.335 \\ 
Akaike Inf. Crit. & 2,854.291 & 2,426.699 & 2,857.907 & 2,428.671 \\ 
\hline 
\hline \\[-1.8ex] 
\textit{Note:}  & \multicolumn{4}{r}{$^{*}$p$<$0.1; $^{**}$p$<$0.05; $^{***}$p$<$0.01} \\ 
\end{tabular} 
\end{table}

\newpage

\section{Survey Text}\label{app:survey_qs}

In this section, we include the text from the survey described in Section~\ref{sec:human-explain}.

\paragraph{Landing page:}

\begin{displayquote}
Welcome to this survey! It was created at the \reviewing{\authorsident}{ \textbf{Combinatorics and Algorithms for Real Problems (CAAR)} Research Experience for Undergraduates (REU)} during the summer of 2021, made possible by the \reviewing{[author's support]}{University of Maryland College Park and the National Science Foundation (NSF)}.

The survey will take approximately approximately 10 minutes to finish. You will be performing two tasks, with each task taking approximately 5 minutes. After finishing the first task, you will be routed to the other task. You may take a short break in between the two tasks, but the survey is intended to be taken in one sitting. If at any time in the middle of a task you need to take a break, be sure to refresh the page.

Once you feel ready, press `Next' to get routed to your first task.
\end{displayquote}

\paragraph{Verification instructions:}

\begin{displayquote}
Welcome to Task A! This task will take approximately 5 minutes. It has 74 questions. Each question will have two images, each of a single face. Your job is to identify whether the faces in these two images are of the same person or not. You can either click on the buttons `Yes' / `No' or press `y' for `Yes' and `n' for `No'. After you click a button or press one of the `y' or `n' keys, you will not be allowed to change your answer, so keep that in mind. Please try to verify whether the two images are of the same person to the best of your ability. If at any time in the middle of a task you need to take a break, be sure to refresh the page. After finishing the last question, you will be directed to Task B. Once you feel ready, click the `Next' button to start this task.
\end{displayquote}

\paragraph{Verification task heading:}

\begin{displayquote}
\textbf{\textit{\underline{Task A:}}} \textbf{Determine whether the following images are of the same person.}
\end{displayquote}

The ``\textbf{\textit{\underline{Task A:}}}" is a link to a popup that displays the verification instructions again.

\paragraph{Identification instructions:}

\begin{displayquote}
Welcome to Task B! This task will take approximately 5 minutes. It has 38 questions. Each question will have ten images, each of a single face. One image will appear on the left of your screen — this is the target image. The other nine images will appear on the right of your screen in a 3-by-3 grid. Exactly one of these nine images will match the identity of the target image. Your job is to click the image in the grid that matches the target. After you click a picture in the gallery, you will not be allowed to change your answer, so keep that in mind. Please try to identify the matching image to the best of your ability. If at any time in the middle of a task you need to take a break, be sure to refresh the page. After finishing the last question, there will be a brief questionnaire asking about your individual information. Once you feel ready, click the `Next' button to start this task.
\end{displayquote}

\paragraph{Identification task heading:}

\begin{displayquote}
\textbf{\textit{\underline{Task B:}}} \textbf{Click the image in the gallery that matches the identity of the target image.}
\end{displayquote}

Similarly, ``\textbf{\textit{\underline{Task B:}}}" is a link to a popup that displays the verification instructions again.

Note that there is a 50-50 chance for starting on verification or identification. In this case, verification was presented first (which is referred to by ``task A") and identification was presented second (which is referred to by ``task B").

\paragraph{User information page:}

\begin{displayquote}
Please enter your information.

All information will be kept strictly private on secure university servers and will be erased after the completion of this study.

Select your age: [0-19, 20-39, 40-59, 60-79, 80+, Prefer not to say]

Select your gender: [Male, Female, Other]

Feel free to elaborate on your gender presentation: [text-box]

Please select the category that best represents your skin tone.

\underline{What are the Fitzpatrick Skin Types?}

[Pale White Skin, White Skin, Light Brown Skin, Moderate Brown Skin, Dark Brown Skin, Deeply Pigmented Dark Brown Skin]
\end{displayquote}

\paragraph{\underline{What are the Fitzpatrick Skin Types?} popup:}

\begin{displayquote}
The \textbf{Fitzpatrick Skin Phototypes} were developed by dermatologist Thomas B. Fitzpatrick. It is a system commonly used to classify skin complexions and their various reactions to exposure to ultraviolet radiation, or sun exposure. There are 6 catogeries, ranging from extremely sensitive skin which always burns instead of tannning, to very resistant skin which is deeply pigmented and almost never burns.
\end{displayquote}

\paragraph{Thanks page:}

\begin{displayquote}
\textbf{Thanks for taking the \reviewing{\authorsident}{REU-CAAR} 2021 Survey!}

Thanks again for finishing the \textbf{\reviewing{\authorsident}{REU-CAAR} 2021} survey! Have a great rest of your day!
\end{displayquote}
