# Supplementary material for: How Technology Impacts and Compares to Humans in Socially Consequential Arenas
Source: arXiv:2211.03554 source file (2022-11-02)
Supplement: Supplementary file 4 [file appendix.tex]

\section{Resubmisison Notes}

This work is a resubmission of a similar paper (with the same title and authors) from the 1st round of the NeurIPS Datasets and Benchmark track. We summarize the concerns of the previous reviewers and outline our significant changes. 

The major change in this version of the paper is the addition of a third API, Google Cloud Platform. We included this third service to address the previous reviewer's concerns about the generalization of our claims regarding the demographic differences. Ultimately, none of our conclusions from Round 1 have been changed with the addition of the third API --- thus offering strong evidence for generalization of our findings and addressing many of the major concerns of the previous reviewers.

R1 (5NTr) provided a final score of 5 (marginally below acceptance threshold). They had two main concerns: (1) we do not address cause and effect, and (2) we did not relate our work to~\citet{hendrycks2019benchmarking}. In this version, we have not addressed (1) following accepted precedent~\citep{grother2010report} and because this question is nearly unanswerable given the level of access we have to third party APIs. R1 agreed with this in their response to our rebuttal. However, we have significantly improved R1's suggestion for comparison to~\citep{hendrycks2019benchmarking}. Among other things, we have included an analysis in Figure~\ref{fig:imagenetc_comp}.

R2 (KtKY) provided a final score of 6 (marginally above acceptance threshold). Their primary concerns were derived from the way in which the results were analyzed and presented. The previous version of our manuscript had a regression for each dataset and service. We have simplified this analysis by only having one regression model for each dataset; this enables more robust comparisons across the services, and we have simplified further by creating a unifying way to compare demographics; see Table~\ref{tbl:comp_full}. As for why we did not have this analysis in the previous submission, we lacked the computing capacity at the time to analyze all the data at once, though we have since acquired the ability and include the updated analysis here. 

R2 also had concerns regarding how robust our metric was. This concern stemmed from our using a classification metric instead of a detection metric. In this version, we have performed a robustness analysis of our metric (starting on line 142) which shows that on the representative subset of data which we fully annotated, our classification metric is highly correlated with the detection metric. 

R3 (3V1x) provided a final score of 6 (marginally above acceptance threshold). Their two concerns centered on the ways in which the corruptions were generated (algorithmically as opposed to naturally) and confusion over the data distributions. We addressed the first concern by highlighting the contrasting possibilities of a small study with natural images or a larger study with reasonable algorithmic corruptions. In the end, the reviewer agreed that our study was meritorious even with the algorithmic corruptions. We then included more clear and concise language about the data distributions.

\section{Evaluation Information}

\subsection{Image Counts}\label{sec:image_counts}

For each dataset, we selected no more than \num{1500} images from any intersectional group. The final tallies of how many images from each group can be found in Tables~\ref{tbl:image_count_breakdown_adience}, \ref{tbl:image_count_breakdown_ccd}, \ref{tbl:image_count_breakdown_miap}, and \ref{tbl:image_count_breakdown_utk}.

{\color{black}
\subsection{Corruption information}

We evaluate 15 corruptions from \citet{hendrycks2019benchmarking}: Gaussian noise, shot noise, impulse noise, defocus blur, glass blur, motion blur, zoom blur, snow, frost, fog, brightness, contrast, elastic transforms, pixelation, and jpeg compressions. Each corruption is described in the \citet{hendrycks2019benchmarking} paper as follows:

The first corruption type is Gaussian noise. This corruption can appear
in low-lighting conditions. Shot noise, also called Poisson noise, is electronic noise caused by the
discrete nature of light itself. Impulse noise is a color analogue of salt-and-pepper noise and can be
caused by bit errors. Defocus blur occurs when an image is out of focus. Frosted Glass Blur appears
with “frosted glass” windows or panels. Motion blur appears when a camera is moving quickly. Zoom
blur occurs when a camera moves toward an object rapidly. Snow is a visually obstructive form of
precipitation. Frost forms when lenses or windows are coated with ice crystals. Fog shrouds objects
and is rendered with the diamond-square algorithm. Brightness varies with daylight intensity. Contrast
can be high or low depending on lighting conditions and the photographed object’s color. Elastic
transformations stretch or contract small image regions. Pixelation occurs when upsampling a lowresolution image. JPEG is a lossy image compression format which introduces compression artifacts.

The specific parameters for each corruption can be found in the project's github at the corruptions file: \url{https://github.com/dooleys/Robustness-Disparities-in-Commercial-Face-Detection/blob/main/code/imagenet_c_big/corruptions.py}.
}

\begin{table}
\caption{\footnotesize Adience Dataset Counts}
\label{tbl:image_count_breakdown_adience}
\centering
\begin{tabular}[t]{llr}
\toprule
     &      &     Count \\
Age & Gender &       \\
\midrule
0-2 & Female &   684 \\
     & Male &   716 \\
3-7 & Female &  1232 \\
     & Male &   925 \\
8-14 & Female &  1353 \\
     & Male &   933 \\
15-24 & Female &  1047 \\
     & Male &   742 \\
25-35 & Female &  1500 \\
     & Male &  1500 \\
36-45 & Female &  1078 \\
     & Male &  1412 \\
46-59 & Female &   436 \\
     & Male &   466 \\
60+ & Female &   428 \\
     & Male &   467 \\
\bottomrule
\end{tabular}
\end{table}

\begin{table}
\centering
\caption{\footnotesize CCD Dataset Counts}
\label{tbl:image_count_breakdown_ccd}
\begin{tabular}{llllr}
\toprule
    &       &       &       &     Count \\
Lighting & Gender & Skin & Age &       \\
\midrule
Bright & Female & Dark & 19-45 &  1500 \\
    &       &       & 45-64 &  1500 \\
    &       &       & 65+ &   547 \\
    &       & Light & 19-45 &  1500 \\
    &       &       & 45-64 &  1500 \\
    &       &       & 65+ &   653 \\
    & Male & Dark & 19-45 &  1500 \\
    &       &       & 45-64 &  1500 \\
    &       &       & 65+ &   384 \\
    &       & Light & 19-45 &  1500 \\
    &       &       & 45-64 &  1500 \\
    &       &       & 65+ &   695 \\
    & Other & Dark & 19-45 &   368 \\
    &       &       & 45-64 &   168 \\
    &       &       & 65+ &    12 \\
    &       & Light & 19-45 &   244 \\
    &       &       & 45-64 &    49 \\
Dim & Female & Dark & 19-45 &  1500 \\
    &       &       & 45-64 &   670 \\
    &       &       & 65+ &   100 \\
    &       & Light & 19-45 &   642 \\
    &       &       & 45-64 &   314 \\
    &       &       & 65+ &   131 \\
    & Male & Dark & 19-45 &  1500 \\
    &       &       & 45-64 &   387 \\
    &       &       & 65+ &    48 \\
    &       & Light & 19-45 &   485 \\
    &       &       & 45-64 &   299 \\
    &       &       & 65+ &   123 \\
    & Other & Dark & 19-45 &    57 \\
    &       &       & 45-64 &    26 \\
    &       &       & 65+ &     3 \\
    &       & Light & 19-45 &    27 \\
    &       &       & 45-64 &    12 \\
\bottomrule
\end{tabular}
\end{table}

\bigskip 

\begin{table}
\caption{\footnotesize MIAP Dataset Counts}
\label{tbl:image_count_breakdown_miap}
\centering
\begin{tabular}{llr}
\toprule
      &         &     Count \\
AgePresentation & GenderPresentation &       \\
\midrule
Young & Unknown &  1500 \\
Middle & Predominantly Feminine &  1500 \\
      & Predominantly Masculine &  1500 \\
      & Unknown &   561 \\
Older & Predominantly Feminine &   209 \\
      & Predominantly Masculine &   748 \\
      & Unknown &    24 \\
Unknown & Predominantly Feminine &   250 \\
      & Predominantly Masculine &   402 \\
      & Unknown &  1500 \\
\bottomrule
\end{tabular}
\end{table}

\begin{table}[!htbp]
\centering
\caption{\footnotesize UTKFace Dataset Counts}
\label{tbl:image_count_breakdown_utk}
\begin{tabular}{lllr}
\toprule
    &      &       &     Count \\
Age & Gender & Race &       \\
\midrule
0-18 & Female & Asian &   555 \\
    &      & Black &   161 \\
    &      & Indian &   350 \\
    &      & Others &   338 \\
    &      & White &   987 \\
    & Male & Asian &   586 \\
    &      & Black &   129 \\
    &      & Indian &   277 \\
    &      & Others &   189 \\
    &      & White &   955 \\
19-45 & Female & Asian &  1273 \\
    &      & Black &  1500 \\
    &      & Indian &  1203 \\
    &      & Others &   575 \\
    &      & White &  1500 \\
    & Male & Asian &   730 \\
    &      & Black &  1499 \\
    &      & Indian &  1264 \\
    &      & Others &   477 \\
    &      & White &  1500 \\
45-64 & Female & Asian &    39 \\
    &      & Black &   206 \\
    &      & Indian &   146 \\
    &      & Others &    22 \\
    &      & White &   802 \\
    & Male & Asian &   180 \\
    &      & Black &   401 \\
    &      & Indian &   653 \\
    &      & Others &    97 \\
    &      & White &  1500 \\
65+ & Female & Asian &    75 \\
    &      & Black &    78 \\
    &      & Indian &    43 \\
    &      & Others &    10 \\
    &      & White &   712 \\
    & Male & Asian &   148 \\
    &      & Black &   166 \\
    &      & Indian &    91 \\
    &      & Others &     5 \\
    &      & White &   682 \\
\bottomrule
\end{tabular}
\end{table}

\section{Metric Discussion}\label{sec:metric_example}

Our use of relative error is slightly adapted from ImageNet-C insomuch that in that paper, they were measuring top-1 error of classification systems. However, the concept is identical. Consequently, it is linguistically best for our measure to be \emph{mean relative} corruption error, whereas ImageNet-C reports the \emph{mean relative} corruption error. This symmantic difference is attributed to when we take our average versus when the ImageNet-C protocol does.

{\color{black}
\subsection{Response Example}\label{sec:response:example}
Our main metric, \mrCE{} relies on the computing the number of detected faces, i.e.,length of a response, $l_r$, from an API service. We explicitly give an example of this here. 

An example response from an API service is below has one face detected:
\begin{lstlisting}
[
  {
    "face_rectangle": {
      "width": 601,
      "height": 859,
      "left": 222,
      "top": 218
    }
  }
]
\end{lstlisting}

An example response from an API service is below has two faces detected:
\begin{lstlisting}
[
  {
    "face_rectangle": {
      "width": 601,
      "height": 859,
      "left": 222,
      "top": 218
    }
  },
  {
    "face_rectangle": {
      "width": 93,
      "height": 120,
      "left": 10,
      "top": 39
    }
  }  
]
\end{lstlisting}

}

\subsection{Metric Example}
Let us consider an example. Assume we were testing the question of whether there is a difference in error rates for different eye colors: (Grey, Hazel, and Brown). Across all the corrupted data, we might see that $\rCE{}$ is 0.12, 0.21, and 0.23 for Grey, Hazel, and Brown respectively. Recall that the odds of an event with likelihood $p$ is reported as $p/(1-p)$. So the odds of error for each eye color is 0.14, 0.27, and 0.30 respectively. Our logistic regression would be written as $\texttt{rCE} = \beta_0 + \beta_1\texttt{Hazel}+\beta_2\texttt{Brown}$, with \texttt{Hazel} and \texttt{Brown} being indicator variables. After fitting our regression, we might see that the estimated \emph{odds} coefficients for the intercept is 0.14, for the variable \texttt{Hazel} is 1.93, and for the variable Brown is 2.14; and all the coefficients are significant. This makes sense because the odds of Grey is 0.14, the odds ratio between Hazel and Grey is 0.27/0.14 = 1.93, and the odds ratio between Brown and Grey is 0.30/0.14 = 2.14. The significance tells us that the odds (or probability) or error for Grey eyes is significantly different from the odds (or probability) of error for Brown and Hazel eyes. In this example, we can conclude that the odds of error is 2.14 higher for Brown eyes compared to Grey. Put another way, for every 1 error for a Grey eyed person, there would be roughly 2 errors for a Hazel or Brown person. More so, the odds of error for Brown eyes is 114\% higher than the odds of error for for Grey eyes.

\section{API Parameteres}\label{sec:api}

For the AWS DetectFaces API,\footnote{\url{https://docs.aws.amazon.com/rekognition/latest/dg/API_DetectFaces.html}} we selected to have all facial attributes returned. This includes age and gender estimates. We evaluate the performance of these estimates in Section \ref{sec:age_gender_prediction}. The Azure Face API\footnote{\url{https://westus.dev.cognitive.microsoft.com/docs/services/563879b61984550e40cbbe8d/operations/563879b61984550f30395236}} allows the user to select one of three detection models. We chose model \texttt{detection\_03} as it was their most recently released model (February 2021) and was described to have the highest performance on small, side, and blurry faces, since it aligns with our benchmark intention. This model does not return age or gender estimates (though model \texttt{detection\_01} does).

\section{Benchmarks Costs}\label{sec:costs}

A total breakdown of costs for this benchmark can be found in Table~\ref{tbl:costs}.

\begin{table}[!htbp]
\centering
\caption{\footnotesize Total Costs of Benchmark}
\label{tbl:costs}
% [inline block 0: 28 envs, 69883 chars -> data_tex | \begin{tabular}{lr} \toprule...]
 }
\end{table}
