# Supplementary material for: How Technology Impacts and Compares to Humans in Socially Consequential Arenas
Source: arXiv:2211.03554 source file (2022-11-02)
Supplement: Supplementary file 5 [file appendices.tex]

\newpage
\appendix

\section{Table of Symbols} \label{app:table of symbols}

We provide in Table \ref{tab:grand_table} for ease of reading and consolidation of all the symbols used in this paper. All the symbols are also defined in main body of the paper. 
\begin{table*}[]
 \centering
\begin{tabular}{c|l}
 \toprule
 Symbols & Description\\
 \midrule
 $A = \{a_i\}_{i=1}^K$ & A set of $K$ arms $a_i$ \\
 $\mu_i$ & Global true utility of arm $a_i$\\
 $\mathcal{S}$ & Set of states of size $S$ \\
 $(s_t)$ & State sequence \\
 $\nu_i$ & Distribution for arm $a_i$ with $\mathbb{E}[\nu_i] = \mu_i$ which draws the $m_{i,s}$ \\
 $m_{i,s}$ & The local, state-based esimate fo the global true utility for arm $a_i$ in state $s$\\
 $\eta_{i,s}$ & Distribution for arm $a_i$ in state $s$ with $\mathbb{E}[\eta_{i,s}]=m_{i,s}$ which determines arm pulls\\
 $X_{i,s}$ & Reward derived from pulling arm $a_i$ in state $s$, $X_{i,s}\sim \eta_{i,s}$\\
 $m_{t}^\ast$ & The highest $m_{i,s}$ at time $t$ \\
 $m_s^\ast$ & The highest $m_{i,s}$ in state $s$ \\
 $i_t^\ast$ & The arm with highest $m_{i,s}$ at time $t$ \\
 $i_s^\ast$ & The arm with highest $m_{i,s}$ in state $s$ \\
 $\overline{R_n}$ & The pseudo-regret of \modelAccro{}\\
 $I_t$ & An allocation strategy\\
 $J_t$ & A recommendation strategy\\
 $N_{i}^s(t)$ & The number of times arm $a_i$ has been pulled in state $s$ by time $t$\\
 $\widehat{m}_{i,s_t,N_i^{s_t}(t)}$ & sample mean for arm $i$ in stage $s_t$ after pulling it $N_i^{s_t}(t)$ times\\
 $\Delta^m_{i,s}$ & The sub-optimality gap of arm $a_i$ in state $s$ defined as $m_s^\ast - m_{i,s}$\\
%  $\Delta_i$ & The smallest $\Delta^m_{i,s}$ across states $s$ for an arm $a_i$; $\min_s \Delta_^m{i,s}$ \\
 $\mu^\ast$ & Global best true utility; the highest $\mu_i$\\
 $j^\ast$ & Global best arm; the arm with highest $\mu_i$\\
 $m^{\hat{\ast}}$ & Empiric best utility estimate; the highest average $m_{i,s}$ across states\\ 
 $j^{\hat{\ast}}$ & Empiric best arm; the arm with highest average $m_{i,s}$ across states\\
 $r_n$ & True simple regret; $r_n = \mu^\ast - \mu_{J_n}$\\
 $\hat{r}_n$ & Empiric simple regret; $\hat{r}_n = m^{\hat{\ast}} - \frac{1}{S}\sum_{s=1}^S m_{J_n,s}$ \\
 ${e}_n$ & The probability that a recommendation strategy does not select $j^{{\ast}}$; $\mathbb{P}(J_n \neq j^{{\ast}})$\\
 $\hat{e}_n$ & The probability that a recommendation strategy does not select $j^{\hat{\ast}}$; $\mathbb{P}(J_n \neq j^{\hat{\ast}})$\\
 $\Delta^\Sigma_i$ & The sub-optimality gap for empiric simple regret; $m^{\hat{\ast}} - \frac{1}{S}\sum_{s=1}^S m_{i,s}$\\
 $\Delta^\mu_i$ & $\mu^\ast - \mu_i$.\\
 $\Sigma_s(t)$ & The number of times $(s_t)$ has been in state $s$ by time $t$ \\

\bottomrule
\end{tabular}
 \caption{List of symbols used with corresponding descriptions and mathematical definitions.}
 \label{tab:grand_table}
\end{table*}

\section{Proof of Theorem \ref{double DAB UCB pseudoregret}}
\begin{proof}
We borrow heavily from the proof of and exposition of Theorem 2.1 in \cite{bubeck2012regret}.

Let $N_i^{s}(n)$ be the number of times the forecaster chose arm $i$ while in state $s$ by the $n^{\text{th}}$ round. Let $\Delta^m_{i,s}=m^\ast_s - m_{i,s}$ be the optimally gap for each arm at each stage.

We observe that we can rewrite the pseudo-regret with these two variables.

{ \begin{align*}
    \overline{R_n} &= \sum_{t=1}^n m^\ast_t - \bbE\left[ \sum_{t=1}^n m_{I_t,s_t} \right]\\
     &= \sum_{s=1}^S\sum_{i=1}^K \bbE[N_i^s(n)]m_s^\ast - \bbE\left[ \sum_{s=1}^S \sum_{i=1}^K N_i^s(n) m_{i,s} \right]\\
     &= \sum_{s,i:\Delta^m_{i,s}>0} \Delta^m_{i,s}\bbE[N_i^s(n)].
\end{align*}}

We now strive to find a bound for this double summation. 
\\

\noindent\textbf{Conditions for choosing to pull arm $i$}

We first observe that if under our Double DAB UCB rule, we choose to pull arm $i$, i.e., $I_t=i$, then one of the three conditions must hold:
{ \begin{align}
    m^\ast_{s_t} &> \widehat{m}_{N_{i^\ast}^{s_t}(t-1)} + (\psi^\ast)^{-1}\left( \frac{\alpha\ln t}{N_{i^\ast}^{s_t}(t-1)} \right) \label{cond-UB}\\
    m_{i,s_t} &< \widehat{m}_{N_{i}^{s_t}(t-1)} -  (\psi^\ast)^{-1}\left(  \frac{\alpha\ln t}{N_i^{s_t}(t-1)}\right) \label{cond-LB}\\
    N_i^{s_t}(t-1) &< \frac{\alpha\ln t}{\psi^\ast(\Delta_{i,s_t}/2)}  \label{not-enough}
\end{align}}

Assume for contradiction that this needn't hold. Then,
{ \begin{align*}
    \widehat{m}_{N_{i^\ast}^{s_t}(t-1)} + (\psi^\ast)^{-1}\left( \frac{\alpha\ln t}{N_{i^\ast}^{s_t}(t-1)} \right) &\geq m^\ast_{s_t}\\
    &= m_{i,s_t} + \Delta_{i,s_t}\\
    &\geq m_{i,s_t} + 2(\psi^\ast)^{-1}\left( \frac{\alpha\ln t}{N_t^{s_t}(t-1)} \right) \\
    &\geq  \widehat{m}_{N_{i}^{s_t}(t-1)} +  (\psi^\ast)^{-1}\left(  \frac{\alpha\ln t}{N_i^{s_t}(t-1)}\right) \label{cond-LB}
\end{align*}}
which yields a contradiction with the chose of the arm $i$.
\\

\noindent\textbf{Detour: Markov's Inequality}

We make a slight detour to prove an important point we will need to anchor the remaining part of our proof. 

We want to put a concentration bound on the deviation of our estimate of $m_{i,s}$ and the true value. Specifically, we will show that for any $x>0$, if $\widehat{m}_{i,s,x}$ is the sample mean of $x$ pulls from the distribution $\eta_{i,s}$ with mean $m_{i,s}$,
{ $$\bbP\left( m_{i,s} - \widehat{m}_{i,s,x} > \epsilon \right) \leq e^{-x\psi^\ast(\epsilon)}$$}

Say that we take $x$ iid samples from $\eta_{i,s}$; denote them as $R_t\sim\eta_{i,s}$ for $t=1,\dots,x$. 
% this is a less rigorous proof 
% https://stats.stackexchange.com/questions/340069/analysing-regret-for-multi-armed-bandits

We now use the Markov inequality to show that for all $\lambda>0$
{ \begin{align*}
    \bbP\left( m_{i,s} - \widehat{m}_{i,s,x} > \epsilon \right) &= \bbP\left( \bbE[R_1] - \frac{1}{x}\sum_{t=1}^x R_t >\epsilon \right)\\
    &= \bbP\left( \sum_{t=1}^x\left(\bbE[R_t] -  R_t\right) > x\epsilon \right)\\
    &\leq \bbE\left[ e^{\lambda\sum_{t=1}^x\left(\bbE[R_t] -  R_t\right)}\right] e^{-x\lambda\epsilon} \\
    &= \bbE\left[ \prod_{t=1}^x e^{\lambda(\bbE[R_t] - R_t)}\right] e^{-x\lambda\epsilon} \\
    &= \prod_{t=1}^x\bbE\left[ e^{\lambda(\bbE[R_t] - R_t)}\right] e^{-x\lambda\epsilon}  \\
    &\leq e^{x\psi(\lambda)-x\lambda\epsilon} = e^{-x(\lambda\epsilon-\psi(\lambda))}
\end{align*}}
Therefore, this inequality also holds for $\psi^\ast(\epsilon) = \sup_{\lambda}(\lambda\epsilon - \psi(\lambda))$.
\\

We now can see that if we set $x=N_i^{s_t}(t-1)$ and $\epsilon = (\psi^\ast)^{-1}\left(\frac{\alpha\ln t}{N_i^{s_t}(t-1)} \right)$, we can put a bound on the probabilities that (\ref{cond-UB}) occurs. 

Observe that for time $t\geq1$, 
{ \begin{align*}
    \bbP \left\{(\ref{cond-UB}) \right\} &\leq \bbP\left\{ \exists x\in\{1,\dots,t-1\} : m^\ast_{s_t} > \widehat{m}_{i^\ast,s,x} + (\psi^\ast)^{-1}\left( \frac{\alpha\ln t}{x} \right)  \right\}\\
    &\leq \sum_{x=1}^t \bbP\left\{ m^\ast_{s_t} - \widehat{m}_{i^\ast,s,x} > (\psi^\ast)^{-1}\left( \frac{\alpha\ln t}{x}\right) \right\}\\
    &\leq \sum_{x=1}^t \frac{1}{t^\alpha} = \frac{1}{t^{\alpha-1}}
\end{align*}}
where the last inequality follows from the Markov inequality proven above. Note, we can use symmetry of this argument for (\ref{cond-LB}).
\\

\noindent\textbf{Bound on $\bbE[N_i^s(n)]$}

We turn back to the main part of the proof, providing a bound on $\bbE[N_i^s(n)]$. 

The core insight is that we have three conditions, one of which must be satisfied to select an arm to pull at time $t$. We observe that condition \ref{not-enough} corresponds to when we choose an arm because it hasn't been pulled enough times. Therefore, we can put $u=\lceil \frac{\alpha\ln(n)}{\psi^\ast(\Delta^m_{i,s}/2)}\rceil$ for some $s$. 

Once an arm has been pulled, if it is chosen to be pulled in the future, then (\ref{cond-UB}) or (\ref{cond-LB}) must be satisfied. So we shall ask for a bound on probabilities of those events. 

{ \begin{align*}
    \bbE[N_i^s(n)] = \bbE\left[\sum_{t=1}^n\mathbb{1}_{\{I_t=i\land s_t=s\}} \right] &\leq u + \sum_{t=u+1}^n\bbP \left\{(\ref{cond-UB}) \right\} + \sum_{t=u+1}^n\bbP \left\{(\ref{cond-LB}) \right\}\\
    &\leq u + 2\sum_{t=u+1}^n \frac{1}{t^{\alpha-1}}\\
    &\leq u + 2\left(1 + \int_1^\infty t^{1-\alpha} dt \right)\\
    &= u + \frac{2}{\alpha-2}\\
    &\leq \frac{\alpha\ln(n)}{\psi^\ast(\Delta^m_{i,s}/2)} + 1+ \frac{2}{\alpha-2} \\
    &= \frac{\alpha\ln(n)}{\psi^\ast(\Delta^m_{i,s}/2)}  + \frac{\alpha}{\alpha-2}
\end{align*}}

We now conclude the proof
{\[
\overline{R_n} = \sum_{s,i:\Delta^m_{i,s}>0} \Delta^m_{i,s}\bbE[N_i^s(n)] \leq  \sum_{s,i : \Delta^m_{i,s}>0} \Delta^m_{i,s}\left[\frac{\alpha\ln(n)}{\psi^\ast(\Delta^m_{i,s}/2)}  + \frac{\alpha}{\alpha-2}\right]
\]}

\end{proof}

\section{Proof of Theorem \ref{Uniform + EBA}}

\begin{proof}
Our goal is obtain an upper bound on the probability that the arm with highest mean of empiric means across the states is \emph{not} equal to $j^{\hat\ast}$. 

Let $J_n$ be the empiric best arm recommendation strategy such that $J_n = \argmax_{i=1,\dots,K} \sum_{s=1}^S \widehat{m}_{N_i^s(n)}$. The intuition behind the proof is to say that, if we can ensure our estimate of the $m_{i,s}$ are tight, i.e., $|m_{i,s} - \widehat{m}_{N_i^s(n)}|<\epsilon_i$ for an appropriately chosen $\epsilon_i$, then we can ensure that we are choosing the right arm. 
\\

Define $B_i$ to be the event:
{ $$B_i = \left\{\left| \frac{1}{S}\sum_{s=1}^S m_{i,s} - \frac{1}{S}\sum_{s=1}^S \widehat{m}_{N_i^s(n)} \right| < \frac{\Delta^\Sigma_i}{2} \right\}.$$ }
Observe that on the event of $\bigcap_{i=1}^K B_i$, we can ensure that the empiric best arm will in fact be $j^{\hat{\ast}}$. This is because the errors for each stage compound linearly. Therefore, $\bigcap_{i=1}^K B_i \subset\{J_n = j^{\hat{\ast}}\}$.

Further, define the event $A_{i,s} = \{\left|m_{i,s} -\widehat{m}_{N_i^s(n)}\right| \geq \frac{\Delta^\Sigma_i}{2} \}$. We see that $\displaystyle\bigcap_{s=1}^S (A_{i,s})^C \subset B_i$ because of the triangle inequality, with 
{ $$\left| \frac{1}{S}\sum_{s=1}^S m_{i,s} - \frac{1}{S}\sum_{s=1}^S \widehat{m}_{N_i^s(n)} \right| \leq \frac{1}{S}\sum_{s=1}^S \left|m_{i,s} - \widehat{m}_{N_i^s(n)} \right| < \frac{\Delta^\Sigma_i}{2}.$$}
So we can re-express $\hat{e}_n$ as a probability of the $A_{i,s}$:
{ \begin{align*}
    \hat{e}_n = \bbP(J_n \neq j^{\hat{\ast}}) &\leq \bbP\left( \left(\bigcap_{i=1}^K B_i\right)^C\right)  \\
    &= \bbP\left( \bigcup_{i=1}^K B_i^C\right) \\
    &= \sum_{i=1}^K\bbP\left(  B_i^C\right) \\
    &\leq \sum_{i=1}^K\bbP\left( \left(\bigcap_{s=1}^S (A_{i,s})^C\right)^C\right)\\
    &= \sum_{i=1}^K \bbP\left(  \bigcup_{s=1}^S A_{i,s}\right)\\
    &\leq \sum_{i=1}^K\sum_{s=1}^S \bbP(A_{i,s})
\end{align*}}

Recall from our proof of Theorem \ref{double DAB UCB pseudoregret}, we can bound the concentration of our estimate $\widehat{m}_{N_i^s(n)}$ by a factor of the number of times its pulled. Concretely, 
{ \begin{align*}
    \bbP(A_{i,s}) &= \bbP(|m_{i,s} - \widehat{m}_{N_i^s(n)} | \geq \Delta^\Sigma_i/2 ) \\
    &\leq \bbP(m_{i,s} - \widehat{m}_{N_i^s(n)}  \geq \Delta^\Sigma_i/2 ) + \bbP(\widehat{m}_{N_i^s(n)} -m_{i,s}  \geq \Delta^\Sigma_i/2 ) \\
    &\leq 2 e^{-N_i^s(n)\psi^\ast(\Delta^\Sigma_i/2)}.
\end{align*}}

With the uniform allocation strategy, we know that for any arm $i$ and state $s$, we have $N_i^s(n) = \lfloor\frac{\Sigma_s(n)}{K}\rfloor$ which allows us to conclude our proof. 

We now turn our attention to the bound on the error in choosing the true best arm. 

Recall that $e_n = \bbP(J_n \neq j^\ast)$, i.e., the probability that the EBA recommendation does not choose the global best arm. 

For each arm $i$ and each stage $s$, put 
{ $$B_{i,s} = \left\{\left| \mu_i - \widehat{m}_{N_i^s(n)} \right| < \frac{\Delta^\mu_i}{2}\right\}.$$}

We see that if this is true for all $i$ and $s$, then 
$\displaystyle\bigcap_{i,s} B_{i,s} \subset \{J_n = j^\ast\}$ by the triangle inequality:
{
\begin{align*}
    |\mu_i - \hat{m}_{N_i^s(n)} | &= \left| \frac{1}{S}\sum_{s=1}^S \mu_i - \frac{1}{S}\sum_{s=1}^S \widehat{m}_{N_i^s(n)} \right| \\
    &\leq \frac{1}{S}\sum_{s=1}^S \left|\mu_{i} - \widehat{m}_{N_i^s(n)} \right| \\
    &< \frac{\Delta^\mu_i}{2}.
\end{align*} 
}

Further, put 
{
\begin{align*}
    A_{i,s} &= \left\{\left| \mu_i - {m}_{i,s} \right| < \frac{\Delta^\mu_i}{4}\right\} \\
    H_{i,s} &= \left\{\left| {m}_{i,s} - \widehat{m}_{N_i^s(n)} \right| < \frac{\Delta^\mu_i}{4}\right\}
\end{align*}
}
We see that, from the triangle inequality, $A_{i,s}\cap H_{i,s} \subset B_{i,s}$, and thus $\displaystyle \bigcap_{i,s}(A_{i,s}\cap H_{i,s}) \subset\{J_n = j^\ast\}$.

\vspace{1em}

We continue by bounding the probability of the complement of $B_{i,s}$. First note, that we can use the triangle inequality to note that

So we can re-express ${e}_n$ as a probability of the $_{i,j}$:
{ 
\begin{align*}
    {e}_n = \bbP(J_n \neq j^{{\ast}}) &\leq \bbP\left( \left(\bigcap_{i,s} \left(A_{i,s}\cap H_{i,s}\right)\right)^C\right)  \\
    &= \bbP\left( \bigcup_{i,s} \left(A_{i,s}^C \cup H_{i,s}^C\right)\right) \\
    &\leq \sum_{i,s}\bbP\left(  A_{i,s}^C\right) + \sum_{i,s}\bbP\left(  H_{i,s}^C\right)     
\end{align*}
}

To bound $A_{i,s}$, we can call upon our assumption of $\nu_i$. Assuming that $\nu_i\sim N(\mu_i,\sigma^2)$, we can compute exactly the probability of $A_{i,s}$ using the cdf of a normal distribution. Precisely, $\bbP(A_{i,s}^C) = 2 \Phi(-(\Delta^\mu_i)/(4\sigma^2))$.

Recall from our proof of Theorem \ref{double DAB UCB pseudoregret}, we can bound the concentration of our estimate $\widehat{m}_{N_i^s(n)}$ by a factor of the number of times its pulled. Concretely, 
{ \begin{align*}
    \bbP(H_{i,s}^C) &= \bbP(|m_{i,s} - \widehat{m}_{N_i^s(n)} | \geq (\Delta^\mu_i)/4 ) \\
    &\leq \bbP(m_{i,s} - \widehat{m}_{N_i^s(n)}  \geq (\Delta^\mu_i)/4 ) + \bbP(\widehat{m}_{N_i^s(n)} -m_{i,s}  \geq (\Delta^\mu_i)/4 ) \\
    &\leq 2 e^{-N_i^s(n)\psi^\ast((\Delta^\mu_i)/4)}.
\end{align*}}

With the uniform allocation strategy, we know that for any arm $i$ and state $s$, we have $N_i^s(n) = \lfloor\frac{\Sigma_s(n)}{K}\rfloor$ which allows us to conclude our proof.

\end{proof}

\section{Proof of Theorem \ref{Uniform + UCB, ETR}}

\begin{proof}
Let us first consider $\bbP(J_n = i)$. For the empiric best arm strategy to choose $i$ at time $n$, i.e., $J_n=i$, it must in particular be true that $\sum_s \widehat{m}_{N_i^{s}(n)} \geq \sum_s \widehat{m}_{N_{j^{\hat{\ast}}}^s(n)}$. We begin by considering the probability that for a given state $s$, we have $\widehat{m}_{N_i^{s}(n)}>\widehat{m}_{N_{j^{\hat{\ast}}}^s(n)}$. If we use Corollary from line 2.11 of \cite{hoeffding1963probability}, we can bound
{ \begin{align*}
    \bbP(\widehat{m}_{N_i^{s}(n)}>\widehat{m}_{N_{j^{\hat{\ast}}}^s(n)}) &= \bbP( \widehat{m}_{N_i^{s}(n)} - \widehat{m}_{N_{j^{\hat{\ast}}}^s(n)} - (m_{i,s} - m_{j^{\hat{\ast}},s}) > (m_{j^{\hat{\ast}},s} - m_{i,s})) \\
    &\leq e^{-\frac{2(m_{j^{\hat{\ast}},s} - m_{i,s})^2}{
    ((N_{j^{\hat{\ast}}}^s(n))^{-1} + (N_i^s(n))^{-1}}}\\
    & = e^{-\lfloor\Sigma_s(n)/K\rfloor(m_{j^{\hat{\ast}},s} - m_{i,s})^2}\\
\end{align*}}
where the last inequality comes from the uniform allocation strategy meaning $N_{j^{\hat{\ast}}}^s(n) = N_i^s(n) = \lfloor\Sigma_s(n)/K\rfloor$.
We now use a union bound to yield the desired result:
{ \begin{align*}
    \bbE[\hat{r}_n] &\leq \sum_{i=1}^K \Delta^\Sigma_i\bbP(J_n = i) \leq \sum_{i=1}^K \Delta^\Sigma_i \sum_{s=1}^S e^{-\lfloor\Sigma_s(n)/K\rfloor(m_{j^{\hat{\ast}},s} - m_{i,s})^2}
\end{align*}}

We can use precisely the same logic as above for the global best arm analysis. 
\end{proof}

\section{Proof of Theorem \ref{SR}}

With the Successive Rejects algorithm, let us compute the number of times each arm is pulled at each time period $t_k$. We see that $N_i^s(t_1) = \lfloor \Sigma_s(t_1) / K\rfloor$ for all $i\in A_1$. Then $N_i^s(t_2) = N_i^s(t_1) + \lfloor (\Sigma_s(t_2)-\Sigma_s(t_{1}))/(K-1)\rfloor$ for all $i\in A_2.$ 
So we conclude that $N_i^s(t_k) = \sum_{\kappa=1}^k \lfloor (\Sigma_s(t_\kappa)-\Sigma_s(t_{\kappa-1}))/(K+1-\kappa)\rfloor$ for all $i\in A_k$.

\begin{proof}
Following the proof of Theorem 2 from \cite{audibert2010best}, assume that the sequence of pulls for every arm in every state is done in advance so we can compare arms pulls that may not have actually happened as the SR algorithm progresses. Assume we are stage $k$ of SR. If $\sum_s \widehat{m}_{i,s,x}$ is rejected in this round, then we know that it must be less than at least one of the $k$ worst arms, i.e., $\sum_s \widehat{m}_{N^s_{j^{\hat{\ast}}}(t_k)} \leq \max_{i\in\{(K),\dots,(K+1-k)} \sum_s\widehat{m}_{N_i^s(t_k)}$. 

Using a union bound as we did in the proof of Theorem \ref{Uniform + UCB, ETR}, we know that 
{ \begin{align*}
    \hat{e}_n &= \bbP(A_K \neq \{j^{\hat{\ast}}\}) \\
    &\leq \sum_{k=1}^{K-1}\sum_{i=K+1-k}^K \sum_{s=1}^S \exp\left\{-\frac{2(m_{j^{\hat{\ast}},s} - m_{(i),s})^2}{
    ((N_{j^{\hat{\ast}}}^s(t_k))^{-1} + (N_{(i)}^s(t_k))^{-1}}\right\}\\
    &= \sum_{k=1}^{K-1}\sum_{i=K+1-k}^K \sum_{s=1}^S \exp\left\{-n_{s,k}(m_{j^{\hat{\ast}},s} - m_{(i),s})^2\right\}\\
    &\leq \sum_{k=1}^{K-1} \sum_{s=1}^S k \exp\left\{-n_{s,k}(m_{j^{\hat{\ast}},s} - m_{(K+1-k),s})^2\right\}
\end{align*}}

We can use precisely the same logic as above for the global best arm analysis. 
\end{proof}
