# Supplementary material for: How Technology Impacts and Compares to Humans in Socially Consequential Arenas
Source: arXiv:2211.03554 source file (2022-11-02)
Supplement: Supplementary file 8 [file appendix.tex]

\section{Table of Variables}

\begin{table}[h]
    \centering
    \small{
    \begin{tabular}{@{}cp{6.5cm}@{}}
    \toprule
        \textbf{Variable} & \textbf{Description} \\
    \midrule
        $S$ & The population of individuals to evaluate. \\
        $n$ & The number of individuals in a population ($|S|=n$). \\
        $a$ & A single individual or arm ($a\in S$).\\
        $u(a)$ & The true risk of an individual. \\
        $\hat{u}(a)$ & The empirical risk of an individual. \\
        $k$ & The number of individuals chosen for clinical intervention. \\
        $k_i$ & The number of individuals to move on to stage $i+1$.\\
        $s_i$ & The information gain of evaluation in stage $i$. \\
        $j_i$ & The cost of evaluation in stage $i$. \\
        $T$ & The total budget. \\
        $T_i$ & The budget for stage $i$. \\
    \bottomrule
    \end{tabular}
    }
    \caption{List of variables used in our approach.}
    \label{tab:vars}
\end{table}

\section{Full Results Table}

The full table of all the results are included in Table \ref{tab:grand_table}.

\begin{table*}[]
 \centering
  \begin{adjustbox}{max width=\textwidth}
\begin{tabular}{l|cc|cccc|cccc}
 \toprule
 Approaches & Budget & \begin{tabular}[c]{@{}c@{}}Number of\\ Individuals\\ Evaluated\end{tabular} & \begin{tabular}[c]{@{}c@{}}Population \\ Sensitivity\end{tabular} & \begin{tabular}[c]{@{}c@{}}Cohort \\ Sensitivity\end{tabular} & Precision & Specificity & \begin{tabular}[c]{@{}c@{}}Cohort \\ TP \end{tabular} & \begin{tabular}[c]{@{}c@{}}Cohort \\ FP\end{tabular} & \begin{tabular}[c]{@{}c@{}}Cohort \\ FN\end{tabular} & \begin{tabular}[c]{@{}c@{}}Cohort \\ TN\end{tabular} \\ \midrule
{\bf NLP-Full} & - & 242 & 0.64 & 0.64 & 0.24 & 0.59 & 27 & 82 & 15 & 118 \\
{\bf NLP-Sub} & - & 100 & 0.27 $\pm$ 0.11 & 0.64 $\pm$ 0.18 & 0.25 $\pm$ 0.10 & 0.59 $\pm$ 0.08 & 11 $\pm$ 4.8 & 34 $\pm$ 7.3 & 6 $\pm$ 3.1 & 49 $\pm$ 7.7 \\
{\bf NLP-Top-100} & - & 242 & 0.55 & 1 & 0.23 & 0 & 23 & 77 & 0 & 0 \\
\midrule
\begin{tabular}[c]{@{}l@{}}\bf{NLP-Top-100} \\ {\bf + 1Expert-Sub}\end{tabular} & \$535 & 242 & 0.49 $\pm$ 0.06 & 0.90 $\pm$ 0.11 & 0.71 $\pm$ 0.10 & 0.89 $\pm$ 0.05 & 21 $\pm$ 2.7 & 9 $\pm$ 3.9 & 2 $\pm$ 2.7 & 68 $\pm$ 3.9 \\
{\bf 1Expert-Sub} & \$535 & 100 & 0.34 $\pm$ 0.03 & 0.91 $\pm$ 0.05 & 0.66 $\pm$ 0.14 & 0.92 $\pm$ 0.05 & 14 $\pm$ 2.3 & 7 $\pm$ 4.3 & 2 $\pm$ 2.3 & 77 $\pm$ 4.3 \\
{\bf MAB} & \$553 & 242 & 0.77 $\pm$ 0.12 & 0.77 $\pm$ 0.12 & 0.33 $\pm$ 0.05 & 0.66 $\pm$ 0.01 & 33 $\pm$ 5.3 & 67 $\pm$ 5.3 & 9 $\pm$ 5.3 & 132 $\pm$ 5.3 \\
{\bf MAB*} & \$553 & 242 & 0.76 $\pm$ 0.13 & 0.76 $\pm$ 0.14 & 0.33 $\pm$ 0.11 & 0.95 $\pm$ 0.03 & 30 $\pm$ 6.0 & 10 $\pm$ 6.2 & 12 $\pm$ 6.0 & 190 $\pm$ 6.2 \\
\midrule
{\bf 1Expert} & \$1,295 & 242 & 0.91 $\pm$ 0.08 & 0.91 $\pm$ 0.08 & 0.67 $\pm$ 0.08 & 0.91 $\pm$ 0.03 & 38 $\pm$ 3.4 & 18 $\pm$ 6.6 & 4 $\pm$ 3.4 & 182 $\pm$ 6.6 \\
{\bf MAB} & \$1,300 & 242 & 0.85 $\pm$ 0.08 & 0.85 $\pm$ 0.08 & 0.36 $\pm$ 0.04 & 0.67 $\pm$ 0.04 & 36 $\pm$ 2.0 & 64 $\pm$ 2.0 & 6 $\pm$ 2.0 & 136 $\pm$ 2.0 \\
{\bf MAB*} & \$1,300 & 242 & 0.74 $\pm$ 0.12 & 0.73 $\pm$ 0.09 & 0.73 $\pm$ 0.08 & 0.95 $\pm$ 0.03 & 31 $\pm$ 4.0 & 11 $\pm$ 6.0 & 11 $\pm$ 4.0 & 189 $\pm$ 6.0 \\
{\bf 4Experts-Sub} & \$2,140 & 100 & 0.43 $\pm$ 0.10 & 1 & 1 & 1 & 18 $\pm$ 4 & 0 & 0 & 82 $\pm$ 4 \\
{\bf MAB} & \$2,200 & 242 & 0.84 $\pm$ 0.03 & 0.84 $\pm$ 0.03 & 0.35 $\pm$ 0.03 & 0.67 $\pm$ 0.01 & 36 $\pm$ 4.0 & 64 $\pm$ 4.0 & 6 $\pm$ 4.0 & 136 $\pm$ 4.0 \\
{\bf MAB*} & \$2,200 & 242 & 0.75 $\pm$ 0.13 & 0.73 $\pm$ 0.14 & 0.74 $\pm$ 0.10 & 0.95 $\pm$ 0.03 & 31 $\pm$ 5.7 & 10 $\pm$ 6.9 & 12 $\pm$ 5.7 & 190 $\pm$ 6.9 \\
{\bf 4Experts} & \$5,179 & 242 & 1 & 1 & 1 & 1 & 42 & 0 & 0 & 200 \\
\bottomrule
\end{tabular}
\end{adjustbox}
 \caption{Main experimental results, organized by budget. Comparisons based on budget should be made across sections in the table; strongest differences are at the lowest budget.  \ignore{Baseline approaches are described in \ref{sec:baselines}. Evaluation protocols are reported in Section \ref{sec:eval}. The three MAB experiments all use the {\bf Linear} encoding mechanism described in Section \ref{sec:encoding}.} For approaches with an element of randomness, means and two standard deviations are reported.}
 \label{tab:grand_table}
\end{table*}

\section{Reproducibility}

\subsection{Data}\label{appendix:data}

In this work, we used the UMD Reddit Suicidality dataset version~2, \url{umiacs.umd.edu/~resnik/umd_reddit_suicidality_dataset.html}, which is available to approved researchers. Note that, owing to the sensitive nature of the data, even though it is anonymous \cite{Benton2017}, access to the dataset requires an application process run by the dataset creators in collaboration with suicide prevention experts at the American Association of Suicidology.

\subsection{NLP Classifier}
\label{sec:training_details}

\begin{figure}[ht!]
  \centering
  \caption{Three-level Hierarchical Attention Network (3HAN)}
  \label{fg:3hanmodel}
\end{figure}

\ignore{We detail our hierarchical attention layer in the context of aggregating a sequence of document vectors to an individual's vector, though the three layers are the same. See Figure~\ref{fg:seq2vec} for an illustration.
For an individual $a$, the $|Q|$ Document vectors $\{d_{a,q}\}_{q=1}^{Q}$ representing the $|Q|$ documents of the individual are first passed through a bi-directional GRU layer. The outputs, after passing through a fully-connected layer and a non-linear layer, are then compared to a learnable attention vector, $v_{\text{attention}}$. Specifically,
\begin{align}
        g_{a,q} &= \text{Bi-GRU}(d_{a,q}) \label{eq:bi_gru}\\
        r_{a,q} &= \text{tanh}\left ( W g_{a,q} + b \right ) \label{eq:transformation_ap}  \\
        \alpha_{a,q} &= \frac{e^{r_{a,q}^\top v_{\text{attention}}}}{\sum_{q^\prime=1}^Q e^{r_{a,q^\prime}^\top v_{\text{attention}}}} \label{eq:atten_ap}\\
        \upsilon_{a} &= \sum\nolimits_{q=1}^Q \alpha_{a,q} g_{a,q} \label{eq:avg_ap}
\end{align}
}

\begin{figure}[ht]
  \centering
  \includegraphics[width=0.8\linewidth]{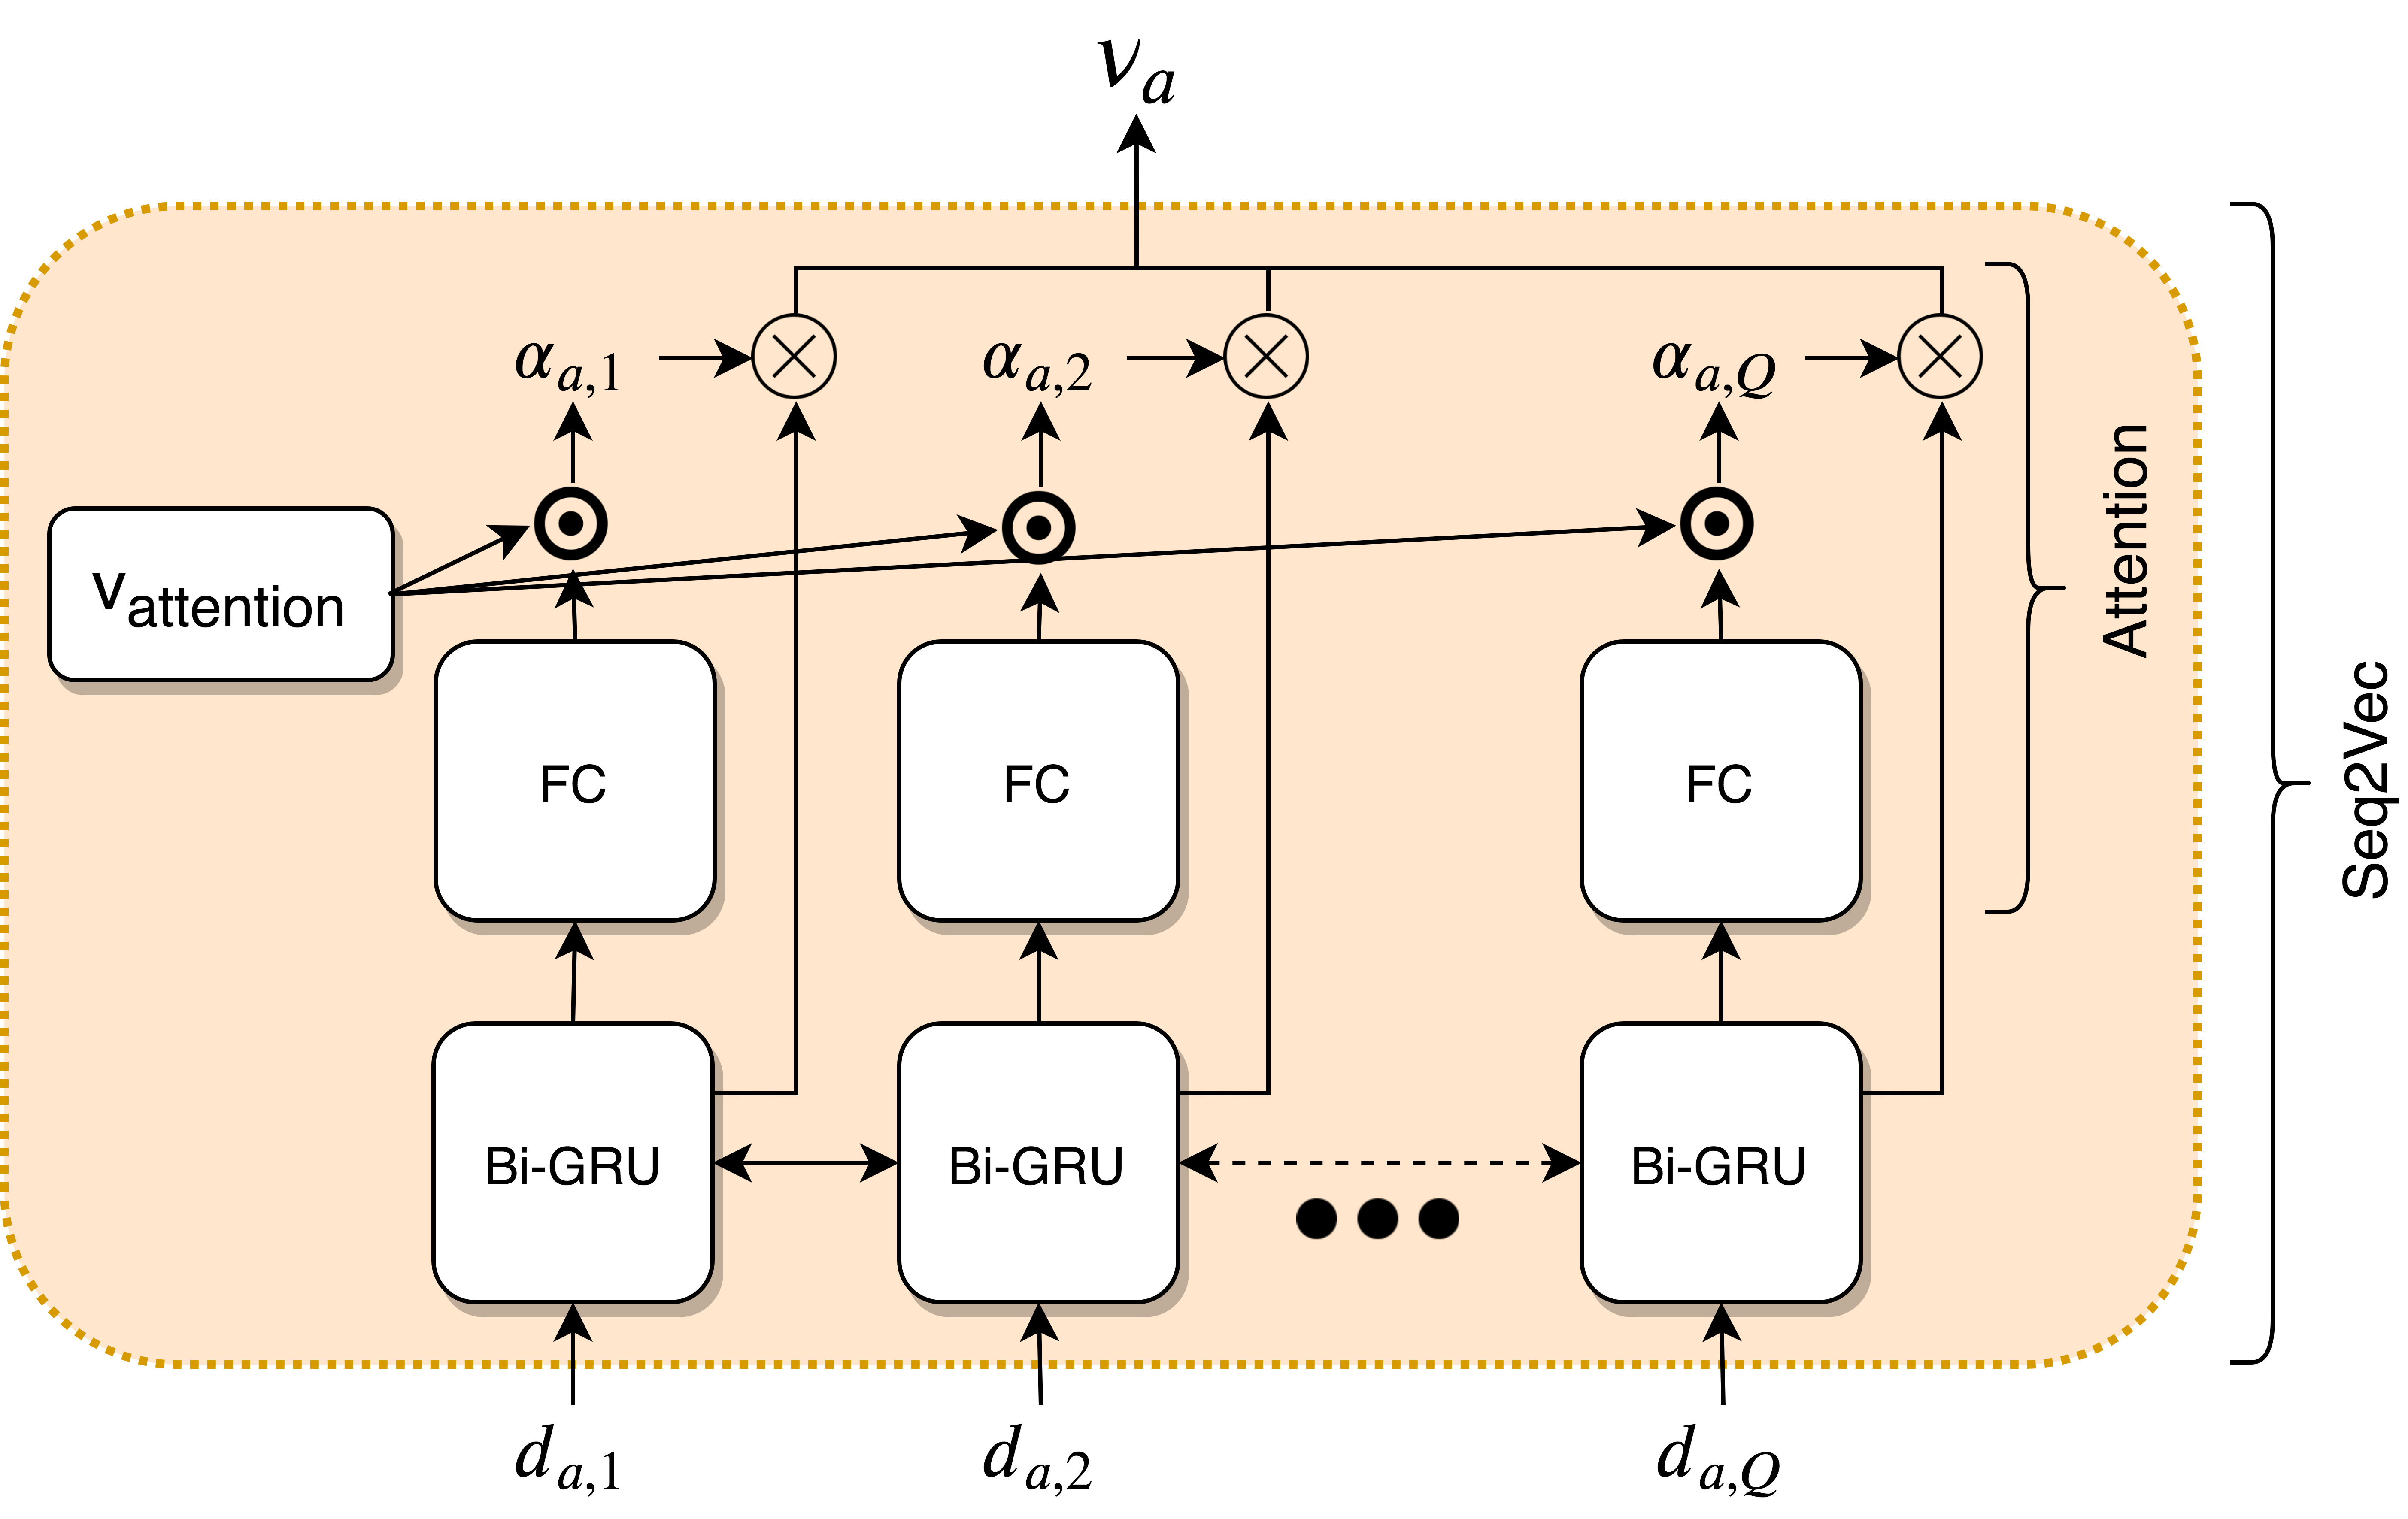}
  \caption{Seq2Vec with Attention}
  \label{fg:seq2vecapp}
\end{figure}

\paragraph{Model.}

Figure~\ref{fg:3hanmodel} illustrates the 3HAN model \cite{shing2020}, which is implemented using AllenNLP~\cite{Gardner2017AllenNLP}.
\textsc{3HAN}'s Seq2Vec layers use bi-directional GRU with attention~\cite{yang2016hierarchical}. For the purpose of reproducibility, we describe the implementation of the hierarchical attention layer in the context of aggregating a sequence of document vectors to an individual's vector, though the three layers are the same (see Figure~\ref{fg:seq2vecapp}).
For an individual $a$, the $|Q|$ Document vectors $\{d_{a,q}\}_{q=1}^{Q}$ representing the $|Q|$ documents of the individual are first passed through a bi-directional GRU layer. The outputs, after passing through a fully-connected layer and a non-linear layer, are then compared to a learnable attention vector, $v_{\text{attention}}$. Specifically,
\begin{align}
        g_{a,q} &= \text{Bi-GRU}(d_{a,q}) \label{eq:bi_gru}\\
        r_{a,q} &= \text{tanh}\left ( W g_{a,q} + b \right ) \label{eq:transformation_ap}  \\
        \alpha_{a,q} &= \frac{e^{r_{a,q}^\top v_{\text{attention}}}}{\sum_{q^\prime=1}^Q e^{r_{a,q^\prime}^\top v_{\text{attention}}}} \label{eq:atten_ap}\\
        \upsilon_{a} &= \sum\nolimits_{q=1}^Q \alpha_{a,q} g_{a,q} \label{eq:avg_ap}
\end{align}

The word-to-sentence layer has input dimension of 200, hidden dimension of 50, and output dimension of 100, since the bi-direction. The sentence-to-document and document-to-individual layer, similarly, has input dimension of 100, hidden dimension of 50, and output dimension of 100.

\paragraph{Training Details.} Tokenization and sentence splitting are done using spaCy~\cite{spacy2}. The \textsc{Crowdsource} dataset is split into a training set (80\%) and a validation set (20\%) for model development. Cross validation on the training set is used for hyperparameter tuning. We did not test on the \textsc{Expert} dataset until all parameters of the models were fixed, and the set of individuals used for training or tuning is disjoint from the 242 individuals used for the MAB experiment..

For training, the word embedding layer of 3HAN is initialized and fixed with the 200-dimensional Glove embedding trained on Twitter~\cite{pennington2014glove}. 3HAN is then pretrained on the binary \textsc{Weak Supervision} dataset from the weak supervision signal of whether the individuals posted on SuicideWatch,  versus the control group of individuals who never posted on any mental health related forums. The model is then further fine-tuned on the moderate quality four-class \textsc{Crowdsource} dataset by transferring the weights (except the last fully-connected prediction layer) over.   We used ADAM with learning rate 0.003, trained for 100 epochs with early stopping on the validation dataset, with early stopping patience set to 30.

\subsection{Running the MAB simulation}

A version of the code can be shared and its use is described below. The dataset has not been included in the supplementary material because of its sensitive nature, but can be accessed as described in Appendix \ref{appendix:data}. We describe the steps to reproduce the experiments assuming the data is available and the machine (i.e. NLP) classifiers have been trained.

At the end of the above steps,  there should be one file with all the human evaluations in them (`human.csv’) and one with the NLP-based predictions for each user (`machine.prediction’). To load these files and create a list of arms, one can run this code:

\begin{lstlisting}
 from RSD import load_RSD
 arms = load_RSD(human_labels=`human.csv',
           NLP_labels=`machine.prediction')
\end{lstlisting}

To run the BRUTaS algorithm, first set up your hyperparameters:

\begin{lstlisting}
 import oracles
 S = [1,10,100]
 J = [1,90,5350]
 K = [200,100,50]
 T = [2,2,2]
 oracle = oracles.c_top_k_oracle
 utility = oracles.top_k_utility
\end{lstlisting}

Then we can instantiate a BRUTaS object and run the algorithm:
\begin{lstlisting}[language=Python]
 from brutas import BRUTaS
 b = BRUTaS(arms, T, K, S, J, oracle,
       utility, oracle_args=[])
 b.run_alg()
\end{lstlisting}

To evaluate, find those arms that made it to the final stage; to do this, one can execute \texttt{b.arm\_stage == 3}. This will facilitate the user in computing any statistics required, using their favorite packages.
